# Supplementary material for: Reinforcement Learning for Scalable and Trustworthy Intelligent Systems
Source: arXiv:2605.08378 source file (2026-05-08)
Supplement: Supplementary file 2 [file ap-appendix_mappo.tex]

\ProvidesFile{ap-appendix_mappo.tex}[2026-04-06 MaPPO appendix]

\chapter{MaPPO Supplementary Results}
\label{app:mappo_supplementary}

\begingroup

\UndefineShortVerb{\|}

\graphicspath{{papers/mappo/}{papers/mappo/figures/}}

\makeatletter
\edef\ZZOldInputPath{\input@path}
\def\input@path{{papers/mappo/}{papers/mappo/appendix/}\ZZOldInputPath}
\@ifundefinedcolor{ForestGreen}{\definecolor{ForestGreen}{rgb}{0.13, 0.55, 0.13}}{}
\@ifundefinedcolor{Apricot}{\definecolor{Apricot}{rgb}{0.98, 0.81, 0.69}}{}
\makeatother

\providecommand{\citep}[1]{\cite{#1}}
\providecommand{\citet}[1]{\cite{#1}}

\section{Theoretical Results}

\subsection{Stationary Convergence of MaPPO}
\label{app:theo_converge}

Recall that 
\begin{equation}
\label{eq:mappo_loss_u}
\begin{aligned}
    \mathcal{L}_{\rm MaP}(\theta) ~=~& 
    \mathop{\mathbb{E}}_{( \mathbf{y}_{w}, \mathbf{y}_{l}, \mathbf{x})\sim\mathcal{D}} \Big[ -\log \sigma \Big( \beta\log \frac{\pi_{\theta}(\mathbf{y}_{w}|\mathbf{x})}{\pi_{\rm ref}(\mathbf{y}_{w}|\mathbf{x})} - \Delta_{r} \beta\log \frac{\pi_{\theta}(\mathbf{y}_{l}|\mathbf{x})}{\pi_{\rm ref}(\mathbf{y}_{l}|\mathbf{x})} \Big)\Big] \\
    ~=~& \mathop{\mathbb{E}}_{( \mathbf{y}_{w}, \mathbf{y}_{l}, \mathbf{x})\sim\mathcal{D}} \Big[ -\log \sigma (u) \Big].
\end{aligned}
\end{equation}

At the first-order stationary point (FOSP), the gradient of the loss with respect to $\theta$ becomes $0$. Thus, we have 
\begin{equation}
\label{eq:mappo_grad_0}
\begin{aligned}
    \nabla \mathcal{L}_{\rm MaP}(\theta) ~=~&
    \mathop{\mathbb{E}}_{( \mathbf{y}_{w}, \mathbf{y}_{l}, \mathbf{x})\sim\mathcal{D}} \Big[ -\beta (1-\sigma(u)) \Big( \nabla \log {\pi_{\theta}(\mathbf{y}_{w}|\mathbf{x})} - \Delta_{r} \nabla \log {\pi_{\theta}(\mathbf{y}_{l}|\mathbf{x})} \Big)\Big] = 0.
\end{aligned}
\end{equation}

Let the optimal policy be $\pi_{\star}$. The above equation holds when 
\begin{equation}
\label{eq:mappo_grad_inside_0}
\begin{aligned}
\nabla \log {\pi_{\star}(\mathbf{y}_{w}|\mathbf{x})} - \Delta_{r} \nabla \log {\pi_{\star}(\mathbf{y}_{l}|\mathbf{x})} ~=~ 0.
\end{aligned}
\end{equation}

Thus, the optimal policy achieves
\begin{equation}
\label{eq:mappo_opt}
\begin{aligned}
\log {\pi_{\star}(\mathbf{y}_{w}|\mathbf{x})} ~=~ \Delta_{r} \log {\pi_{\star}(\mathbf{y}_{l}|\mathbf{x})} + c,
\end{aligned}
\end{equation}
where $c$ is a scaling constant determined by the initialization. Thus, the model learns a stable log-linear relationship between preferred and less-preferred responses, scaled by the prior reward gap.

In DPO, the optimal policy at the FOSP is
\begin{equation}
\label{eq:dpo_opt}
\begin{aligned}
\log {\pi_{\star}(\mathbf{y}_{w}|\mathbf{x})} ~=~ \log {\pi_{\star}(\mathbf{y}_{l}|\mathbf{x})} + c.
\end{aligned}
\end{equation}
DPO converges to maximizing the log-odds between $\mathbf{y}_{w}$ and $\mathbf{y}_{l}$, but no inherent bound on the preference gap, which can lead to confidence degeneration. 
As training progresses, DPO may tend to decrease the likelihood of both $\mathbf{y}_{w}$ and $\mathbf{y}_{l}$ (the \emph{squeezing effect}), because there is no constraint on absolute probabilities -- only the relative gap matters.

MaPPO prevents overconfidence and instability by grounding optimization in the reward-based prior. 
The FOSP of MaPPO guarantees a bounded, calibrated log-probability ratio between $\mathbf{y}_{w}$ and $\mathbf{y}_{l}$. 
Naturally limits the \emph{squeezing effect} by scaling the impact of $\mathbf{y}_{l}$ via $\Delta_{r}$.
Therefore, MaPPO is theoretically more stable, especially for near-tie preference pairs and in large models where DPO can exacerbate miscalibration.

%%%%%%%%%%%%%%%%%%%%%%%%%%%%%%%%%%%%%%%%
\subsection{Lipschitz Stability}
\label{app:Lipschitz}

First, we list the standard assumptions for the analysis.
\begin{assumption}{\ }
\label{assum:bound}
\begin{enumerate}
% \item The norm of the score function is bounded as $\left\|\nabla \log \pi_\theta (\mathbf{y} | \mathbf{x}) \right\| \leq M$.
\item The score function is Lipschitz continuous as $\left\|\nabla \log \pi_\theta (\mathbf{y} | \mathbf{x}) - \nabla \log \pi_{\theta'} (\mathbf{y} | \mathbf{x}) \right\| \leq M_{g}$.
\end{enumerate}
\end{assumption}

Let the gradient operator be defined as
\begin{equation}
\label{eq:lip_mappo}
\begin{aligned}
\tau_{\theta} ~\coloneqq~  \nabla \mathcal{L}_{\rm MaP}(\theta).
\end{aligned}
\end{equation}

Then, the gradient operator $\tau$ is Lipschitz continuous with
\begin{equation}
\label{eq:lip_bound_mappo}
\begin{aligned}
\| \tau_{\theta} - \tau_{\theta'} \| \le L_{\rm MaP} \| \theta - \theta' \|,
\end{aligned}
\end{equation}
where $L_{\rm MaP} = \beta (1 - \sigma(u)) (1 + \Delta_{r}) M_{g} < \beta (1 + \Delta_{r}) M_{g}$.

\begin{proof}
We have
\begin{equation}
\begin{aligned}
\tau_{\theta} ~=~ -\beta (1-\sigma(u)) \Big( \nabla \log {\pi_{\theta}(\mathbf{y}_{w}|\mathbf{x})} - \Delta_{r} \nabla \log {\pi_{\theta}(\mathbf{y}_{l}|\mathbf{x})} \Big).
\end{aligned}
\end{equation}

The norm of the gradient difference is 
\begin{equation}
\begin{aligned}
\| \tau_{\theta} - \tau_{\theta'} \| ~=&~ \beta (1-\sigma(u)) \cdot \| \nabla \log {\pi_{\theta}(\mathbf{y}_{w}|\mathbf{x})} - \nabla \log {\pi_{\theta'}(\mathbf{y}_{w}|\mathbf{x})} \| \\
&+ \beta (1-\sigma(u)) \Delta_{r} \cdot \| \nabla \log {\pi_{\theta}(\mathbf{y}_{l}|\mathbf{x})} - \nabla \log {\pi_{\theta'}(\mathbf{y}_{l}|\mathbf{x})} \|.
\end{aligned}
\end{equation}

We have that $\sigma(u)$ is Lipschitz with constant $\frac{1}{4}$. Combining the $M_{g}$ Lipschitz of the score function $\nabla \log \pi_\theta (\mathbf{y} | \mathbf{x})$, we have
\begin{equation}
\begin{aligned}
\| \tau_{\theta} - \tau_{\theta'} \| \leq \beta (1 - \sigma(u)) (1 + \Delta_{r}) M_{g} \| \theta - \theta' \| ~\coloneqq~ L_{\rm MaP} \| \theta - \theta' \|.
\end{aligned}
\end{equation}
\end{proof}

In contrast, in DPO, the gradient is Lipschitz continuous as
\begin{equation}
\label{eq:lip_bound_dpo}
\begin{aligned}
\| \tau_{\theta} - \tau_{\theta'} \| \le L_{\rm DPO} \| \theta - \theta' \|,
\end{aligned}
\end{equation}
where $L_{\rm DPO} = 2\beta (1 - \sigma(u)) M_{g} < 2\beta M_{g}$. The Lipschitz constant of the gradients in DPO is larger than that in MaPPO, which shows the gradients have less stability in DPO.

With a formal upper bound on MaPPO's gradient variation, we show a clear theoretical justification for why MaPPO is less prone to instability and exploding confidence gaps, compared to DPO.
\clearpage
\newpage
\section{Supplementary Examples}
\label{app:Supplementary_Examples}

\begin{figure}[!htbp]
\begin{tcolorbox}[title=Prompt~$\mathbf{x}$,fonttitle=\bfseries, boxrule=0.5mm]
Solve the following math problem step-by-step. Simplify your answer as much as possible. Present your final answer as \boxed{Your Answer}. If the sum of two positive integers is 22 and the difference of their squares is 44, what is the product of the two integers?
\end{tcolorbox}
\end{figure}

%%%%%%%%%%%%%%%%%%%%%%%%%%%%%%%%%%%%%%%%
\newpage
\subsection{Before Preference Optimization}
\begin{figure}[!htbp]
\begin{tcolorbox}[colback=green!5, colframe=black!60!green!45, title={\textbf{Response}~$\mathbf{y}_{w}$, $r=0.93$}, fonttitle=\bfseries, boxrule=0.5mm]
To solve this problem step-by-step, let's denote the two positive integers as \(x\) and \(y\) with \(x > y\).

Step 1: Set Up Equations

~~~~Given:

~~~~~~~~1. The sum of the two integers: \(x + y = 22\)

~~~~~~~~2. The difference of their squares: \(x^2 - y^2 = 44\)

Step 2: Factorize the Difference of Squares
Recall that the difference of squares can be factored as:
\[ x^2 - y^2 = (x + y)(x - y) \]
Substitute the given sum \(x + y = 22\) into the factored form:
\[ 44 = 22(x - y) \]

Step 3: Solve for \(x - y\)
Divide both sides by 22:
\[ x - y = 2 \]

Step 4: Solve the System of Linear Equations
Now, we have the system:
1. \(x + y = 22\)
2. \(x - y = 2\)

Add these two equations to eliminate \(y\):
\[ (x + y) + (x - y) = 22 + 2 \]
\[ 2x = 24 \]
\[ x = 12 \]

Substitute \(x = 12\) back into the first equation to find \(y\):
\[ 12 + y = 22 \]
\[ y = 10 \]

Step 5: Calculate the Product
The product of the two integers \(x\) and \(y\) is:
\[ x \cdot y = 12 \cdot 10 = 120 \]

Final Answer
\[ \boxed{120} \] 
\end{tcolorbox}
\end{figure}

\begin{figure}[!htbp]
\begin{tcolorbox}[colback=red!5, colframe=black!60!red!45, title={\textbf{Response}~$\mathbf{y}_{l}$, $r=0.90$}, fonttitle=\bfseries, boxrule=0.5mm]
To solve this problem step-by-step, let's denote the two positive integers as \(x\) and \(y\), where \(x > y\). We are given two conditions:

1. The sum of the two integers is 22:
   \[ x + y = 22 \]

2. The difference of their squares is 44:
   \[ x^2 - y^2 = 44 \]

We can use the identity for the difference of squares, \(x^2 - y^2 = (x + y)(x - y)\), to rewrite the second equation. Substituting \(x + y = 22\) into the identity gives:
\[
(x + y)(x - y) = 44 \implies 22(x - y) = 44
\]
Dividing both sides by 22:
\[
x - y = 2
\]

Now we have a system of linear equations:
\[
\begin{cases}
x + y = 22 \\
x - y = 2
\end{cases}
\]

Adding these two equations eliminates \(y\):
\[
(x + y) + (x - y) = 22 + 2 \implies 2x = 24 \implies x = 12
\]

Substituting \(x = 12\) back into the first equation to solve for \(y\):
\[
12 + y = 22 \implies y = 10
\]

Thus, the two integers are \(x = 12\) and \(y = 10\).

To find the product of the two integers:
\[ xy = 12 \times 10 = 120 \]

Therefore, the product of the two integers is \boxed{120}. 
\end{tcolorbox}
\begin{center}
\caption{Before MLE optimization, the model consistently generates high-quality (high rewards) answers $\mathbf{y}_{w}$ and $\mathbf{y}_{l}$ with prompt $\mathbf{x}$.}
\end{center}
\end{figure}

%%%%%%%%%%%%%%%%%%%%%%%%%%%%%%%%%%%%%%%%%%%
\clearpage
\newpage
\subsection{After MLE Optimization}

\begin{figure}[!htbp]
\begin{tcolorbox}[breakable,colback=green!5, colframe=black!60!green!45, title={\textbf{Response}~$\mathbf{y}_{w}$, $r=0.87$}, fonttitle=\bfseries, boxrule=0.5mm]
To solve the given problem, we'll proceed through the following steps systematically:

Given:

~~~~1. The sum of two positive integers \( x \) and \( y \) is 22.

~~~~2. The difference of their squares is 44.

We need to determine the product of these two integers.

Step-by-Step Solution:

1. Setting up Equations:
   
   - From the first condition: 
     \[
     x + y = 22
     \]
   - From the second condition (expressing the difference of squares):
     \[
     x^2 - y^2 = 44
     \]
   
   We know that \( x^2 - y^2 \) can be factored using the difference of squares formula:
     \[
     x^2 - y^2 = (x+y)(x-y)
     \]

2. Substitute \( x + y \):
   
   - Using the known value from equation (1) in the factored form of the difference of squares:
     \[
     x^2 - y^2 = (x+y)(x-y) \implies 44 = 22(x-y)
     \]
   - Solve for \( x - y \):
     \[
     22(x - y) = 44 \implies x - y = 2
     \]

3. Solving the System of Linear Equations:
   
   - Now, we have the system of equations:
     \[
     x + y = 22
     \]
     \[
     x - y = 2
     \]
   - Add these two equations to eliminate \( y \):
     \[
     (x + y) + (x - y) = 22 + 2
     \]
     \[
     2x = 24 \implies x = 12
     \]
   - Substitute \( x = 12 \) back into \( x + y = 22 \) to find \( y \):
     \[
     12 + y = 22 \implies y = 10
     \]
\end{tcolorbox}
\end{figure}

\clearpage
\newpage
\begin{figure}[!htbp]
\begin{tcolorbox}[breakable,colback=green!5, colframe=black!60!green!45, title={\textbf{Response}~$\mathbf{y}_{w}$, $r=0.87$}, fonttitle=\bfseries, boxrule=0.5mm]
4. Finding the Product:
   
   - With \( x = 12 \) and \( y = 10 \), calculate the product:
     \[
     xy = 12 \times 10 = 120
     \]

Thus, the product of the two integers is \boxed{120}.
\end{tcolorbox}
\end{figure}

\begin{figure}[!htbp]
\begin{tcolorbox}[colback=red!5, colframe=black!60!red!45, title={\textbf{Response}~$\mathbf{y}_{l}$, $r=0.43$}, fonttitle=\bfseries, boxrule=0.5mm]
Step 1: Interpret the problem and set up equations based on the given information.
Given that the sum of two positive integers is 22 and the difference of their squares is 44, we need to find these integers and subsequently their product.

Let's denote the two integers as \(a\) and \(b\) such that \(a > b\), to simplify handling the difference and sum relationships given directly without specifying which integer represents \(a\) or \(b\) in terms of being greater than the other directly addresses addressing conditions related directly to interpreting the context regarding how the operations (sum, difference of squares) relate between two specified integers, based on the given descriptions for solving in the context presented, focusing on correctly interpreting and directly addressing the specific requirements as outlined for accurately proceeding with solving based on the given details, to correctly proceed according to provided instructions and the nature of solving based on the specifications given for dealing with the described conditions around the operation outcomes involving the integers in question.
\[ \]
Step 2: Translate the given conditions into mathematical equations.

~~~~- The sum of the two integers equals 22: \(a + b = 22\).

~~~~- The difference of their squares equals 44: \(a^2 - b^2 = 44\).
\[ \]
Step 3: Utilize algebraic identities for simplification.
From the second equation, apply the algebraic identity for the difference of squares: 
\[a^2 - b^2 = (a + b)(a - b)\]
Thus, substituting in the known value for \(a + b\):
\[(a + b)(a - b) = 44 \implies 22(a - b) = 44.\]

Step 4: Solve for \(a - b\).
Divide both sides by 22:
\[a - b = 2.\]

Step 5: Solve the system of linear equations.
We now have two simultaneous equations:

~~~~1. \(a + b = 22\)

~~~~2. \(a - b = 2\)

Add the two equations together to eliminate \(b\):
\[(a + b) + (a - b) = 22 + 2 \implies 2a = 24 \implies a = 12.\]
\end{tcolorbox}
\end{figure}

\clearpage
\newpage
\begin{figure}[!htbp]
\begin{tcolorbox}[colback=red!5, colframe=black!60!red!45, title={\textbf{Response}~$\mathbf{y}_{l}$, $r=0.43$}, fonttitle=\bfseries, boxrule=0.5mm]
Substitute \(a = 12\) back into the first equation to solve for \(b\):
\[12 + b = 22 \implies b = 10.\]

Step 6: Find the product of \(a\) and \(b\).
The product of the two integers \(a\) and \(b\) is:
\[ab = 12 \times 10 = 120.\]

Step 7: Box the final answer.
\[\boxed{120}\]

\end{tcolorbox}
\begin{center}
\caption{After MLE optimization, the model degenerates, and the outputs $\mathbf{y}_{w}$ and $\mathbf{y}_{l}$ become verbose (low rewards) with prompt $\mathbf{x}$.}
\end{center}
\end{figure}

\clearpage
\newpage
\subsection{After MaP Optimization}

\begin{figure}[!htbp]
\begin{tcolorbox}[colback=green!5, colframe=black!60!green!45, title={\textbf{Response}~$\mathbf{y}_{w}$, $r=0.94$}, fonttitle=\bfseries, boxrule=0.5mm]
To solve this problem step-by-step, let's denote the two positive integers by \(x\) and \(y\), where without loss of generality, we assume \(x > y\).

Given:

~~~~1. The sum of the two integers: \(x + y = 22\)

~~~~2. The difference of their squares: \(x^2 - y^2 = 44\)
\[\]
Step 1: Express the Difference of Squares

~~~~We know from algebra that:
\[ x^2 - y^2 = (x + y)(x - y) \]

~~~~Given \(x + y = 22\), we substitute this into the equation:
\[ 44 = 22(x - y) \]

Step 2: Solve for \(x - y\)

~~~~Divide both sides by 22:
\[ x - y = 2 \]

Step 3: Solve the System of Linear Equations

~~~~Now, we have a system of linear equations:

~~~~~~~~1. \(x + y = 22\)

~~~~~~~~2. \(x - y = 2\)

~~~~Add these two equations to eliminate \(y\):
\[ (x + y) + (x - y) = 22 + 2 \]
\[ 2x = 24 \]
\[ x = 12 \]

~~~~Subtract the second equation from the first to eliminate \(x\):
\[ (x + y) - (x - y) = 22 - 2 \]
\[ 2y = 20 \]
\[ y = 10 \]
\end{tcolorbox}
\end{figure}

\clearpage
\newpage
\begin{figure}[!htbp]
\begin{tcolorbox}[colback=green!5, colframe=black!60!green!45, title={\textbf{Response}~$\mathbf{y}_{w}$, $r=0.94$}, fonttitle=\bfseries, boxrule=0.5mm]
Step 4: Calculate the Product of the Two Integers

~~~~Now that we have \(x = 12\) and \(y = 10\), we find their product:
\[ xy = 12 \times 10 = 120 \]

~~~~Thus, the product of the two integers is:
\[\boxed{120}\]
\end{tcolorbox}
\end{figure}

\begin{figure}[!htbp]
\begin{tcolorbox}[colback=red!5, colframe=black!60!red!45, title={\textbf{Response}~$\mathbf{y}_{l}$, $r=0.88$}, fonttitle=\bfseries, boxrule=0.5mm]
To solve this problem, we'll use algebraic methods to represent the given conditions and then solve for the integers. Here are the steps:

1. Define Variables:
   
~~~~Let the two positive integers be \(x\) and \(y\), with \(x > y\).
\[\]
2. Set Up Equations Based on Given Information:
   
~~~~- The sum of the two integers is 22:
     \[
     x + y = 22
     \]
   
~~~~- The difference of their squares is 44:
     \[
     x^2 - y^2 = 44
     \]

3. Factor the Difference of Squares:
   
~~~~Recall that \(x^2 - y^2\) can be factored as \((x + y)(x - y)\). Therefore:
   \[
   (x + y)(x - y) = 44
   \]
~~~~Substitute \(x + y = 22\) into the equation:
   \[
   22(x - y) = 44
   \]

4. Solve for \(x - y\):
   
~~~~Divide both sides by 22:
   \[
   x - y = 2
   \]
\end{tcolorbox}
\end{figure}

\clearpage
\newpage
\begin{figure}[!htbp]
\begin{tcolorbox}[colback=red!5, colframe=black!60!red!45, title={\textbf{Response}~$\mathbf{y}_{l}$, $r=0.88$}, fonttitle=\bfseries, boxrule=0.5mm]
5. Set Up a System of Linear Equations:

~~~~We now have the system:
   \[
   \begin{cases}
   x + y = 22 \\
   x - y = 2
   \end{cases}
   \]

6. Add the Two Equations to Solve for \(x\):

~~~~Adding the equations eliminates \(y\):
   \[
   (x + y) + (x - y) = 22 + 2
   \]
~~~~Simplifies to:
   \[
   2x = 24 \implies x = 12
   \]

7. Substitute \(x = 12\) Back to Find \(y\):
   
~~~~Using \(x + y = 22\):
   \[
   12 + y = 22 \implies y = 10
   \]

8. Calculate the Product of the Two Integers:

~~~~The product of \(x\) and \(y\) is:
   \[
   x \cdot y = 12 \cdot 10 = 120
   \]
The answer is
 \[\boxed{120}\]

\end{tcolorbox}
\begin{center}
\caption{After MaP optimization, the model consistently generates high quality outputs with prompt $\mathbf{x}$.}
\end{center}
\end{figure}
\clearpage
\newpage
\section{Supplementary Experiments}
\label{app:Experiments}

\subsection{Supplementary Experimental Settings}
\label{mappo:sec:app_exp_setting}

\paragraph{Hyperparameter settings.} 
We follow the standard settings and list the hyperparameter details in the training process of MaPPO in Table \ref{table:hyper}. 
We keep the hyperparameter settings for different model series and model sizes, including Qwen2.5-\{1.5B, 3B, 7B\}-Instruct, Mistral-7B-Instruct, and Llama-3-8B-Instruct models. 

\begin{table}[!htbp]
\caption{Hyperparameter settings in MaPPO.}
\centering
 % \small
\label{table:hyper}
\begin{tabular}{l|lc}
\toprule[1.1pt]
% \hline
{Hyperparameter} & {Value} & {} \\
\midrule[1.1pt]
{global batch size} & {$128$} & { } \\
{learning rate $\eta$} & {$5\times 10^{-7}$} & { } \\
{warmup steps} & {$100$} & { } \\
{weight decay} & {$0.01$} & { } \\
{optimizer} & {AdamW} & { } \\
{KL weight $\beta$} & {$0.1$} & { } \\
{number of responses $n$} & {$8$} & { } \\
{temperature $T$} & {$1.0$} & { } \\
{precision} & {${\tt bfloat16}$} & { } \\
\bottomrule[1.1pt]
\end{tabular}
\end{table}

\begin{table}[!htbp]
\caption{Hyperparameter settings in DPO Variants.}
\centering
 % \small
\label{table:hyper_variants}
\begin{tabular}{l|lc}
\toprule[1.1pt]
{Hyperparameter} & {Value} & {} \\
\midrule[1.1pt]
{SimPO: $\gamma$} & {$1$} & { } \\
{IPO: $\beta$} & {$0.1$} & { } \\
{CPO: $\lambda$} & {$0.2$} & { } \\
\bottomrule[1.1pt]
\end{tabular}
\end{table}

In Table \ref{table:hyper_variants}, we list the extra hyperparameters in the reproduce of the DPO variants. 
The other hyperparameter settings keep the same in Table \ref{table:hyper}. 
Notably, we choose nearly the best hyperparameters for the other methods, and our reproduction achieves higher performances than the original or other reproduction reports on some benchmarks, \textit{e.g.}, SimPO on Arena-Hard. 

\paragraph{Computing Resources.} 
All tasks are trained and evaluated on a platform with $8$ NVIDIA A100 GPUs on each node, and $80$ GB of memory for each GPU. 
Each training task requires between $4$ and $20$ hours to execute, depending on the size of the model.

\subsection{Supplementary Results}
\label{mappo:app:supp_results}

\paragraph{Ablation Study on RMs.} 
As illustrated in Eq.~\ref{eq:prior_prob}, the prior is instantiated via a reward model (RM).
To better understand the role of RMs, we conduct an ablation study by integrating different open-source RMs into our framework, including BT model\footnote{https://huggingface.co/sfairXC/FsfairX-LLaMA3-RM-v0.1}, MoE model\footnote{https://huggingface.co/RLHFlow/ArmoRM-Llama3-8B-v0.1}, and uncertainty-aware model\footnote{https://huggingface.co/LxzGordon/URM-LLaMa-3.1-8B}. As shown in Table~\ref{table:RewardAblation_app}, the absolute performance of I-DPO varies considerably depending on the chosen RM. Importantly, across all settings, our proposed MaPPO plugin consistently boosts performance on AlpacaEval 2.0, Arena-Hard, and MT-Bench. These results highlight two key insights: (i) the choice of RM can influence the strength of supervision and the final outcomes, and (ii) MaPPO is robust to such variation, reliably enhancing DPO regardless of the underlying RM. This robustness underscores the generality and flexibility of our framework.

\begin{table}[!ht]
% \vspace{-4mm}
\caption{Ablation on reward models. $\uparrow$ indicates the higher the better.}
\centering
\label{table:RewardAblation_app}
\resizebox{\textwidth}{!}{%
\begin{tabular}{l|l|l|lll}
\toprule[1.1pt]
{Model} & {Reward Model} & {Method} & {AlpacaEval 2.0 $\uparrow$} & {Arena-Hard $\uparrow$} & {MT-Bench $\uparrow$} \\
\midrule[1.1pt]

\multirow{9}{*}{Qwen2.5-7B-IT}  
& \multirow{3}{*}{sfairXC/FsfairX-LLaMA3-RM-v0.1} 
& {IT} & {$27.03$}  & {$42.9$ }  & {$8.61$ } \\
& & {I-DPO} & {$33.80$} & {$46.9$} & {$\mathbf{8.55}$}\\
& & {+\textbf{MaPPO}} & {$\mathbf{39.10}$ $\textcolor{ForestGreen}{+5.30}$} & {$\mathbf{61.6}$ $\textcolor{ForestGreen}{+14.7}$} & {$8.54$ $\textcolor{Apricot}{-0.01}$}\\
\cline{2-6}
{}
& \multirow{3}{*}{RLHFlow/ArmoRM-Llama3-8B-v0.1} 
& {IT} & {$27.03$}  & {$42.9$ }  & {$8.61$ } \\
& & {I-DPO} & {$28.79$} & {$48.3$} & {$8.58$}\\
& & {+\textbf{MaPPO}} & {$\mathbf{31.56}$ $\textcolor{ForestGreen}{+2.77}$} & {$\mathbf{52.0}$ $\textcolor{ForestGreen}{+3.7}$} & {$\mathbf{8.60}$ $\textcolor{ForestGreen}{+0.02}$}\\

\cline{2-6}
{}  
& \multirow{3}{*}{LxzGordon/URM-LLaMa-3.1-8B} 
& {IT} & {$27.03$}  & {$42.9$ }  & {$8.61$ } \\
& & {I-DPO} & {$32.26$} & {$55.1$} & {$8.60$}\\
& & {+\textbf{MaPPO}} & {$\mathbf{36.17}$ $\textcolor{ForestGreen}{+3.91}$} & {$\mathbf{59.4}$ $\textcolor{ForestGreen}{+4.3}$} & {$\mathbf{8.62}$ $\textcolor{ForestGreen}{+0.02}$}\\

\midrule[1.1pt]

\multirow{9}{*}{Llama-3-8B-IT}  
& \multirow{3}{*}{sfairXC/FsfairX-LLaMA3-RM-v0.1} 
& {IT} & {$10.85$} &{$10.2$}&{$7.52$}\\
& & {I-DPO} & {${29.47}$} &{$25.6$ }&{$8.01$}\\
& & {+\textbf{MaPPO}} & {$\mathbf{32.68}$ $\textcolor{ForestGreen}{+3.21}$} & {$\mathbf{31.0}$ $\textcolor{ForestGreen}{+5.4}$} & {$\mathbf{8.04}$ $\textcolor{ForestGreen}{+0.03}$} \\
\cline{2-6}
{}  
& \multirow{3}{*}{RLHFlow/ArmoRM-Llama3-8B-v0.1} 
& {IT} & {$10.85$} &{$10.2$}&{$7.52$}\\
& & {I-DPO} & {$12.69$} &{$8.1$ }&{$7.44$}\\
& & {+\textbf{MaPPO}} & {$\mathbf{16.69}$ $\textcolor{ForestGreen}{+4.00}$} & {$\mathbf{16.4}$ $\textcolor{ForestGreen}{+8.3}$} & {$\mathbf{7.78}$ $\textcolor{ForestGreen}{+0.34}$} \\

\cline{2-6}
{}  
& \multirow{3}{*}{LxzGordon/URM-LLaMa-3.1-8B} 
& {IT} & {$10.85$} &{$10.2$}&{$7.52$}\\
& & {I-DPO} & {$25.61$} &{$30.4$ }&{$8.06$}\\
& & {+\textbf{MaPPO}} & {$\mathbf{27.83}$ $\textcolor{ForestGreen}{+2.22}$} & {$\mathbf{33.7}$ $\textcolor{ForestGreen}{+3.3}$} & {$\mathbf{8.10}$ $\textcolor{ForestGreen}{+0.04}$} \\

\bottomrule[1.1pt]
\end{tabular}
} % end resizebox
\end{table}

\begin{table}[!ht]
% \vspace{-4mm}
\caption{Comparison w/wo SFT-B and w/wo MaPPO. $\uparrow$ indicates the higher the better.}
\centering
  \small
\label{table:EvaluationICLR_app}
\begin{tabular}{l|l|lll}
\toprule[1.1pt]
% \hline
{Model} & {Method} & {AlpacaEval 2.0 $\uparrow$} & {Arena-Hard $\uparrow$} & {MT-Bench $\uparrow$} \\
\midrule[1.1pt]
\multirow{5}{*}{Qwen2.5-7B-IT} & {IT} & {$27.03$}  & {$42.9$ }  & {$8.61$ } \\
\cline{2-5}
{ } & {I-DPO} & {$33.80$} & {$46.9$} & {$\mathbf{8.55}$}\\
{ } & {+\textbf{MaPPO}} & {$\mathbf{39.10}$ $\textcolor{ForestGreen}{+5.30}$ ~$\textcolor{blue}{+5.30}$} & {$\mathbf{61.6}$ $\textcolor{ForestGreen}{+14.7}$ $\textcolor{blue}{+14.7}$} & {$8.54$ $\textcolor{Apricot}{-0.01}$ $\textcolor{blue}{-0.01}$} \\
\cline{2-5}
{ } & {+\textbf{SFT-B}} & {$51.36$\ \ $\textcolor{ForestGreen}{+17.56}$} & {$33.5$\ \ $\textcolor{Apricot}{-13.4}$} & {$8.01$ $\textcolor{Apricot}{-0.54}$} \\
{ } & {+\textbf{+MaPPO}} & {$\textbf{55.84}$ $\textcolor{ForestGreen}{+22.04}$ $\textcolor{blue}{+4.48}$} & {$\mathbf{43.5}$ ~$\textcolor{Apricot}{-3.4}$ ~$\textcolor{blue}{+10.0}$} & {$\mathbf{8.40}$ $\textcolor{Apricot}{-0.15}$ $\textcolor{blue}{+0.39}$}\\
\midrule[1.1pt]
\multirow{5}{*}{Llama-3-8B-IT} & {IT} & {$10.85$} &{$10.2$}&{$7.52$}\\
\cline{2-5}
{ } & {I-DPO} & {${29.47}$} &{$25.6$}&{$8.01$} \\
{ } & {+\textbf{MaPPO}} & {$\mathbf{32.68}$ $\textcolor{ForestGreen}{+3.21}$ $\textcolor{blue}{+3.21}$} & {$\mathbf{31.0}$ $\textcolor{ForestGreen}{+5.4}$ $\textcolor{blue}{+5.4}$} & {$\mathbf{8.04}$ $\textcolor{ForestGreen}{+0.03}$ $\textcolor{blue}{+0.03}$} \\
\cline{2-5}
{ } & {+\textbf{SFT-B}} & {$35.55$ ~$\textcolor{ForestGreen}{+6.08}$} & {$30.1$ ~$\textcolor{ForestGreen}{+4.5}$} & {$8.02$ ~$\textcolor{ForestGreen}{+0.01}$} \\
{ } & {+\textbf{+MaPPO}} & {$\mathbf{36.21}$ $\textcolor{ForestGreen}{+6.74}$ $\textcolor{blue}{+0.66}$} & {$\mathbf{31.5}$ $\textcolor{ForestGreen}{+5.9}$ $\textcolor{blue}{+1.4}$} & {$\mathbf{8.03}$ $\textcolor{ForestGreen}{+0.02}$ $\textcolor{blue}{+0.01}$} \\
\bottomrule[1.1pt]
\end{tabular}
\end{table}

\paragraph{Comparison with Other Methods.} 
We also compare our approach with complementary techniques, such as the method proposed by \cite{ren2024learning}, which introduces an additional SFT-based pre-processing (denoted as SFT-B) to mitigate the squeezing effect.
It is worthy to mention that our proposed method is compatible with SFT-B.

In Table~\ref{table:EvaluationICLR_app}, we use the \textcolor{blue}{blue} color to indicate the improvement with the MaPPO plugin, and the \textcolor{ForestGreen}{green} color to indicate the improvement compared to I-DPO. 
We find SFT-B alone can bring substantial gains in certain metrics but may also introduce trade-offs on others (e.g., lower Arena-Hard performance on Qwen2.5-7B). By contrast, when combined with MaPPO, the two methods operate jointly and achieve consistent improvements across most benchmarks. These findings demonstrate that MaPPO can be seamlessly integrated with diverse training strategies, further broadening its applicability in practice.

\section{Further Discussions}
\label{app:Discussions}

%%%%%%%%%%%%%%%%%%%%%%%%%%%%%%%%%%%%%%%%
\subsection{Prior Function}
\label{app:Prior_Function}

In Bayes estimation, the prior distribution is usually constructed by experts with domain knowledge without an exception to avoid it \citep{jaynes2007prior}.
We choose a simple form in \eqref{eq:prior_prob}, which has the same structure as the widely used prior function \citep{blei2010probabilistic} and aligns with the softmax probability. 
This brings a very clean result in \eqref{eq:mappo_loss}.
In this paper, we offer an effective function with good performances and concise formulation.
We bring the MaP design into the DPO pipeline, and the prior function construction is not the aim of this paper.
Other function choices that are designed by domain experts are also acceptable and open to be used.

On the other hand, we perform ablation studies on reward models in Appendix \ref{mappo:app:supp_results}, which shows the robustness to different reward signals.

%%%%%%%%%%%%%%%%%%%%%%%%%%%%%%%%%%%%%%%%
\subsection{Recent RL Methods}
\label{app:rl_methods}

In addition to the methods discussed in the introduction section, several recent variants of RL methods for LLMs further contextualize the landscape in which PO operates. 
DAPO \citep{yu2025dapo} introduces a scalable RL system that integrates data selection, clip-higher, overlong reward shaping, and token-level loss into a unified framework, demonstrating strong empirical performance at scale. 
GSPO \citep{zheng2025group} generalizes sequence-level policy optimization to groupwise preference structures, enabling the use of ranked or collectively generated signals and thereby broadening the applicability of RL methods into mixture-of-experts (MoE) architectures. 
PRO \citep{guo2025proximalized} proposes a proximalized formulation of preference optimization that decomposes preference signals into stable update components, allowing the method to accommodate diverse feedback modalities while improving optimization stability. 
Together, these approaches represent the most recent advances in preference optimization and RL post-training, situating MaPPO alongside them highlights its complementary role as a principled, prior-informed extension that remains compatible with the post-training pipelines. 
An interesting direction for future work is exploring how prior knowledge can be integrated into these RL methods.

\DefineShortVerb{\|}

\endgroup
