# Supplementary material for: Reinforcement Learning for Scalable and Trustworthy Intelligent Systems
Source: arXiv:2605.08378 source file (2026-05-08)
Supplement: Supplementary file 7 [file appendix_questions.tex]

\section{\textcolor{blue}{Additional Discussions}}
\label{app:Additional_Discussions}

In this section, we add some Q\&A from the rebuttal period, which may help to clarify the raised questions.

\textbf{Q1:} \textit{In Table 2, DeepSeek-R1-Distill-Qwen-14B originally has higher utility than the instruction-tuned Qwen 14B, but after RL training the utility lowered significantly. This much decrease due to RL is not seen in the IT models in Table 1. What could be happening?}

The key reason lies in the initial behavior of the DeepSeek-R1-Distill-Qwen-14B model prior to RL training. As shown in Table~\ref{tab:llm_lrm}, this model tends to disclose \emph{all} information - both required and restricted attributes - in its outputs. This behavior yields very high utility scores but results in low integrity and complete scores. In the extreme case, a model that always reveals all attributes would achieve $100\%$ utility but $0\%$ integrity and complete.

After applying CI-RL, the model learns to withhold restricted attributes, which leads to significant improvements in both integrity and complete metrics. However, this shift in behavior naturally causes a modest drop in utility, as the model becomes more cautious overall.

In contrast, the instruction-tuned (IT) models in Table~1 start from a more balanced behavior: they do not aggressively disclose all available information, and thus have relatively higher integrity and complete scores even before RL. Because their initial utility is lower (due to more conservative sharing), RL training can improve CI adherence while maintaining or even slightly improving utility.

As an additional point regarding the initial behavior of the DeepSeek-R1-Distill-Qwen-14B model, we note that DeepSeek-R1-Distill-Qwen-14B is primarily optimized for reasoning in scientific and technical domains at the expense of broader domain coverage, whereas our synthetic dataset covers diverse, real-world contexts (e.g., hospitality, education, family) that may fall outside its distributional strengths. This domain mismatch could further contribute to the model’s lower task completion performance under CI constraints initially.

\textbf{Q2:} \textit{Compare with other methods, such as AirGapAgent (CCS24) \citep{Bagdasarian2024AirGapAgent}.}

We regard AirGapAgent as a valuable and timely contribution to the study of privacy-aware LLM agents. AirGapAgent restricts access to private information by prompting an off-the-shelf LLM to decide which inputs are strictly necessary for task completion. In this sense, it shares conceptual similarities with our CI-CoT prompting approach, where a model reasons explicitly about which attributes to use or withhold based on CI.

While we agree that a more direct comparison would be informative, it is unfortunately not feasible at this time. To the best of our knowledge, neither the code nor the dataset for AirGapAgent has been released, and the paper does not report results on standardized benchmarks such as PrivacyLens or ConfAIde. This makes a head-to-head comparison under controlled conditions difficult.

Nonetheless, we view our work as complementary: AirGapAgent enforces privacy via task-specific prompting to limit information exposure, while our work focuses on training models — via both prompting (CI-CoT) and reinforcement learning (CI-RL) — to internalize generalizable CI norms. 
% We are happy to discuss AirGapAgent in more detail in the related work section to highlight these connections and distinctions.
