# Supplementary material for: Reinforcement Learning for Scalable and Trustworthy Intelligent Systems
Source: arXiv:2605.08378 source file (2026-05-08)
Supplement: Supplementary file 8 [file appendix_related.tex]

\section{Supplementary Related Work}
\label{app:related_work}

\paragraph{Chain-of-Thought (CoT) Prompting.} CoT prompting was first proposed by~\citet{wei2022chain}, who demonstrated that having the model articulate its reasoning step by step substantially boosts LLMs' performance on complex reasoning tasks.
Since then, an extensive and rapidly expanding literature has refined CoT decoding, explored structured searches over reasoning paths, distilled rationales into smaller models, and examined faithfulness and safety concerns. 
Owing to the sheer breadth of these follow-up efforts, we simply direct the reader to the comprehensive survey on CoT reasoning~\citep{chu2024navigateenigmaticlabyrinthsurvey} for a detailed taxonomy and coverage of the field.

\paragraph{RL Post-Training of LLMs.}
PPO~\citep{schulman2017proximal} and its variants such as GRPO~\citep{shao2024deepseekmath} have recently shown great success in producing high-performing reasoning models, also known as large reasoning models (LRMs)~\citep{jaech2024openai, guo2025deepseek}. 
Reinforcement learning (RL) post-training has been applied across a wide range of domains, e.g., math~\citep{shao2024deepseekmath}, visual generation~\citep{yan2025rlgf, zhang2024seppo}, and explainable agents~\citep{liu2025utility}, making comprehensive citation of all relevant work infeasible. Therefore, we refer the readers to recent surveys and the references therein~\citep{xu2025largereasoningmodelssurvey, tie2025surveyposttraininglargelanguage, kumar2025llmposttrainingdeepdive, wu2025preference}.

\paragraph{Reasoning and Safety.}
H-CoT \citep{kuo2025h} injects execution-phase thoughts, and bypasses safety checks embedded in chain-of-thought reasoning.
The results reveal a critical vulnerability in LRMs, such as OpenAI's o1/o3, DeepSeek-R1, and Gemini 2.0, in which they can be manipulated to produce harmful content.
With a two-stage training process, GuardReasoner \citep{liu2025guardreasoner} designs a guard model that enhances safety by guiding language models to reason explicitly during moderation tasks.
\citet{kumar2025overthink} proposes an indirect prompt injection attack that stealthily forces reasoning LLMs to generate excessive reasoning tokens into untrusted external contexts used during inference.
SafeChain \citep{jiang2025safechain} studies the safety risks posed by LRMs that generate long CoT outputs. It reveals that such reasoning traces can still include unsafe content despite correct final answers.
ThinkGuard \citep{wen2025thinkguard} proposes a critique-augmented safety guardrail model that improves the safety and interpretability of LLMs by incorporating step-by-step reasoning into safety classification.
BoT \citep{zhu2025bot} designs a backdoor attack that disrupts the intrinsic reasoning mechanisms of o1-like LLMs by inserting stealthy triggers that force models to skip their long-thought processes.

While contextual integrity (CI) encompasses aspects of safety, these works primarily address how LLMs respond to unsafe queries, whereas our work focuses on maintaining contextual integrity within the given context. Thus, these works take an orthogonal direction to ours.
