# Supplementary material for: Reinforcement Learning for Scalable and Trustworthy Intelligent Systems
Source: arXiv:2605.08378 source file (2026-05-08)
Supplement: Supplementary file 9 [file appendix_results.tex]

\section{Supplementary Results}
\label{sec:supplementary_results}

% \paragraph{Ablation Study of KL Divergence Weight.}
% In Table \ref{tab:kl}, we show the ablation results of the KL divergence weight $\beta$ in \eqref{eq:grpo_loss} in our tasks and on the PrivacyLens benchmark. In general, over large $\beta$ damages both privacy and utility performance, and relatively smaller $\beta$ leads to higher privacy rate, but slightly lower utility rate.

% \begin{table}[ht]
%     \centering
%     \caption{Ablation Results of the KL Divergence Weight $\beta$}
%     \input{tables/kl.tex}
%     \label{tab:kl}
% \end{table}

\paragraph{Integrity-utility trade-off via reward function design.}
We conduct this ablation using the model Qwen2.5-7B-Instruct.
We introduce two new parameters $\alpha$ and $\gamma$ to adjust the weighting of required and restricted keywords in the reward function defined in Equation~\eqref{eq:reward}:
\begin{equation}
R =
\begin{cases}
-1 & \text{if the response violates the required format} \\
\alpha \frac{|A_{\text{present}}|}{|A|} - \gamma \frac{|D_{\text{present}}|}{|D|} & \text{otherwise}
\end{cases} \; .
\label{eq:reward2}
\end{equation}
% \begin{equation}
% R =
% \begin{cases}
% -1 & \text{if the response violates the required format} \\
% \alpha \sum\limits_{a \in A_{\text{present}}} \frac{1}{|A|} - \gamma \sum\limits_{d \in D_{\text{present}}} \frac{1}{|D|} & \text{otherwise}
% \end{cases}
% \label{eq:reward2}
% \end{equation}
In Table \ref{tab:reward_function}, we show the results of integrity-utility trade-off with different reward designs in Equation~\eqref{eq:reward2}. {The definitions of helpfulness, LR, and ALR are introduced in Section 
\ref{sec:PrivacyLens} regarding the PrivacyLens benchmark.}

\begin{table}[ht]
    \centering
    \caption{Integrity-utility trade-off with various reward function designs. }
    \begin{tabular}{l|ccc|ccc}
    \toprule
    ($\alpha$, $\gamma$) & $\mathcal{I}$ (in \%) $\uparrow$ & $\mathcal{U}$ (in \%) $\uparrow$ & $\mathcal{C}$ (in \%) $\uparrow$ & LR $\downarrow$ & ALR $\downarrow$ & Helpful [0-3] $\uparrow$ \\
    \midrule
    (1, 0.25) & 71.9 & 71.9 & 48.4 & 38.5 & 39.3 & 2.12 \\
    (1, 0.5) & 78.1 & 76.6 & 59.4 & 35.7 & 38.6 & 2.02 \\
    (1, 1) & 75.0 & 67.2 & 48.4 & 33.7 & 33.9 & 2.08 \\
    (0.5, 1) & 79.7 & 71.9 & 57.8 & 34.1 & 36.1 & 1.98 \\
    (0.25, 1) & 82.8 & 68.8 & 57.8 & 32.3 & 35.3 & 2.01 \\
    \bottomrule
\end{tabular}
    \label{tab:reward_function}
\end{table}

The results demonstrate that placing greater weight on required keywords (\(\alpha\)) generally improves utility—both in terms of task performance and Helpfulness—across our setting and the PrivacyLens benchmark. 
Conversely, increasing the weight on restricted keywords (\(\gamma\)) leads to improved integrity scores and reduced leakage, as reflected by lower leakage rates (LR) and adjusted leakage rates (ALR) in percentage ($\%$) in both evaluation settings.

%%%%%%%%%%%%%%%%%%%%%%%%%%%%%%%%%%%%%%%%%%%%%%%%%%%%%
\paragraph{ConfAIde Benchmark.}
We have additionally evaluated our CI-RL-trained Qwen2.5-7B-Instruct model on the ConfAIde \citep{mireshghallah2024can} benchmark. Our results show that CI-RL also leads to meaningful improvements on ConfAIde, further validating the generality of our approach.

\begin{table}[ht]
    \centering
    \caption{Pearson’s correlation between human and model judgments for Tier 1, Tier 2.a, and Tier 2.b, higher values show more agreement.}
    \begin{tabular}{lc|cc|cc|cc}
        \toprule
        \multicolumn{2}{l}{Model} & \multicolumn{2}{|c}{Tier 1 $\uparrow$} &  \multicolumn{2}{c}{Tier 2.a $\uparrow$} & \multicolumn{2}{c}{Tier 2.b $\uparrow$} \\
        \midrule
        Qwen2.5-7B-Instruct & \color{PineGreen}{+ \textbf{CI-RL}} & 0.58 & \color{PineGreen}{\textbf{0.67}} & 0.51 & \color{PineGreen}{\textbf{0.69}} & 0.48 & \color{PineGreen}{\textbf{0.48}} \\
        \bottomrule
    \end{tabular}
\label{tab:confaide1}
\end{table}

Table~\ref{tab:confaide1} demonstrates that our CI-RL approach leads to improved correlation between human and model judgments across Tier 1 and Tier 2, which evaluates the basic ability to understand the sensitivity of a given information and expectations of information flow within context.

\begin{table}[ht]
    \centering
    \caption{Results for Tier 3: Theory of mind as context. The leakage rate of model generations for contextually appropriate responses and handling private information within a more nuanced scenario involving three parties.}
    \begin{tabular}{lc|cc}
        \toprule
        \multicolumn{2}{l}{Model} & \multicolumn{2}{|c}{Leakage thru. string match $\downarrow$} \\
        \midrule
        Qwen2.5-7B-Instruct & \color{PineGreen}{+ \textbf{CI-RL}} & 0.91 & \color{PineGreen}{\textbf{0.52}}  \\
        \bottomrule
    \end{tabular}
\label{tab:confaide2}
\end{table}

In the next tier (Tier 3), the evaluation focuses on the model’s ability to regulate the disclosure of private information in more complex, multi-party scenarios. Unlike the earlier tiers, which primarily assess a model's capacity to judge the appropriateness of given information flows, this tier examines whether the model can generate contextually appropriate responses that demonstrate an implicit understanding of others' perspectives—an ability related to theory of mind.
Once again, as shown in Table~\ref{tab:confaide2}, our CI-RL approach yields a substantial reduction in the leakage of private information in the model’s responses.

\begin{table}[ht]
    \centering
    \caption{Results for Tier 4: Private and public information flow. The metrics evaluate the privacy reasoning of LLMs in terms of their ability
to discern private (leaks secret) and public information (omits info), when presented with both types in a single scenario. Lower is better for all metrics.}
    \begin{tabular}{lc|cc|cc|cc}
        \toprule
        \multicolumn{2}{l}{Model} & \multicolumn{2}{|c}{Leaks Secret $\downarrow$} &  \multicolumn{2}{c}{Omits Info $\downarrow$} & \multicolumn{2}{c}{Leaks Secr or Omits Info $\downarrow$} \\
        \midrule
        Qwen2.5-7B-IT & \color{PineGreen}{+ \textbf{CI-RL}} & 0.80 & \color{PineGreen}{\textbf{0.30}} & 0.10 & \color{PineGreen}{\textbf{0.15}} & 0.85 & \color{PineGreen}{\textbf{0.45}} \\
        \bottomrule
    \end{tabular}
\label{tab:confaide3}
\end{table}

Table~\ref{tab:confaide3} reports the results of the metrics where models are used as AI meeting assistants generating a meeting summary, in which it is important to exclude a particular sensitive information from the discussion, while including the vital public information.
Finally, we observe that our CI-RL approach significantly improves task completion while adhering to CI constraints - reducing the rate of completions that either leak a secret or omit required information from $0.85$ to $0.45$.

%%%%%%%%%%%%%%%%%%%%%%%%%%%%%%%%%%%%%%%%%%%%%%%%%%%%%%%%%%
% \subsection{Results on Academic Benchmarks}

% Post-training in a certain domain may have negative effects on general reasoning, calibration, and generating accurate responses \citep{NEURIPS2022_b1efde53, bai2022training}. Thus, in Table \ref{tab:academic_bench}, we test the model performance on six widely used benchmarks after our CI-optimized RL training with different model scales. The tasks includes explicit instruction following (IFEval) \citep{zhou2023instruction}, general knowledge (GPQA) \citep{rein2024gpqa}, multitask language understanding (MMLU) \citep{hendrycks2021measuring}, commonsense reasoning (HellaSwag) \citep{zellers-etal-2019-hellaswag}, human falsehoods mimicking (TruthfulQA) \citep{lin-etal-2022-truthfulqa}, and math problem solving (GSM8K) \citep{cobbe2021training}.

% \begin{table}[ht]
%     \centering
%     \caption{Model performance on academic benchmarks}
%     \input{tables/academic_bench.tex}
%     \label{tab:academic_bench}
% \end{table}

%%%%%%%%%%%%%%%%%%%%%%%%%%%%%%%%%%%%%%%%%%%%%%%%%%%%%%
% \paragraph{Evaluation results on ConfAIde.}

%%%%%%%%%%%%%%%%%%%%%%%%%%%%%%%%%%%%%%%%%%%%%%%%%%%%%%
% \paragraph{Method comparison.}
