# Supplementary material for: Reinforcement Learning for Scalable and Trustworthy Intelligent Systems
Source: arXiv:2605.08378 source file (2026-05-08)
Supplement: Supplementary file 10 [file appendix_setting.tex]

\section{Supplementary Details in Experiments}
\label{sec:append_Hyperparameters}

\paragraph{Hyperparameters.}
Sampling a batch of queries with batch size $B=32$, we take $G=16$ inference results on each query from the current policy model, and calculate the rule-based rewards according to Equation \eqref{eq:reward} on each result. 
With $B$ groups of rewards $r$, we optimize the policy $\pi_{\theta}$ by maximizing the GRPO objective function in Equation \eqref{eq:grpo_loss}. 
To maximize the objective, we use the gradient ascent method with mini-batch size $128$, \textit{i.e.}, $32\times 16/128=4$ steps for each GRPO update. 

We use a learning rate $1\times 10^{-6}$ without warmup steps, and a KL divergence weight $\beta=0.001$ by default.
We set the clip ratio $\epsilon=0.2$. The entropy penalty is $0$.
The maximum response length is set to $2048$, and the temperature in LLM sampling is set to $0.7$ in the training process.

%%%%%%%%%%%%%%%%%%%%%%%%%%%%%%%%%%%%%%%%%%%%%%%%%%%%%
\paragraph{Synthetic Data.}

We provide a summary of key dataset statistics in Table~\ref{tab:data-stats} and Table~\ref{tab:attr-stats}. 
The dataset spans $9$ applications and $3$ privacy principles, with no extreme imbalance.
Each synthetic instruction includes on average $2.73$ allowed and $2.08$ disallowed personal attributes, drawn from $526$ and $322$ unique attribute types respectively, illustrating substantial lexical diversity and coverage.
{For synthetic data generation in Section \ref{sec:dataset}, the temperature is set to $0.7$ to encourage diverse but coherent outputs.}

Regarding the verification of instructions for avoiding obvious cues, we conducted a manual audit of randomly sampled instances, and found that they adhere to CI expectations and scenario consistency.

%---------------------------  DATASET STATISTICS  ---------------------------
\begin{table}[ht]
\centering
% \small
\caption{Statistics of our \textbf{synthetic dataset} ($n=729$).}
\label{tab:data-stats}
\begin{tabular}{lrr}
\toprule
\textbf{Application Domain} & \textbf{\#} & \textbf{\%} \\
\midrule
Healthcare      & 143 & 19.6 \\
Hospitality     & 100 & 13.7 \\
Family          &  87 & 11.9 \\
Education       &  78 & 10.7 \\
Finance         &  74 & 10.2 \\
Entertainment   &  73 & 10.0 \\
Friends         &  69 &  9.5 \\
Government      &  67 &  9.2 \\
eCommerce       &  38 &  5.2 \\
\midrule
\textbf{Privacy Principle} & & \\
Confidentiality & 428 & 58.7 \\
Proportionality & 201 & 27.6 \\
Consent         & 100 & 13.7 \\
\bottomrule
\end{tabular}
\end{table}

\begin{table}[ht]
\centering
% \small
\caption{Size of the \emph{allowed} vs.\ \emph{disallowed} attribute
lists per example and the vocabulary covered by the entire dataset.}
\label{tab:attr-stats}
\begin{tabular}{lrrrrrrr}
\toprule
& \textbf{Min} & \textbf{Max} & \textbf{Mean} & \textbf{Median} & \textbf{Unique} \\
\midrule
Allowed     & 1 & 5 & 2.73 & 3 & 526 \\
Disallowed  & 1 & 3 & 2.08 & 2 & 322 \\
\bottomrule
\end{tabular}
\end{table}

%%%%%%%%%%%%%%%%%%%%%%%%%%%%%%%%%%%%%%%%%%%%%%%%%%%%%
\paragraph{Output Lengths in PrivacyLens Evaluation.}

We ran statistics on the number of output tokens produced by the CI-RL-trained model over the PrivacyLens benchmark. The distribution is as follows:
\begin{itemize}[left=0pt]
    \item \textbf{Minimum:} 60 tokens
    \item \textbf{Maximum:} 836 tokens
    \item \textbf{Mean:} 244.72 tokens
    \item \textbf{Standard deviation:} 126.44 tokens
\end{itemize}

These results suggest that while the output lengths vary with task complexity, the overall response length remains moderate. We note that our reward function does not explicitly encourage longer outputs; in fact, CI-RL often leads to more focused completions by discouraging unnecessary or privacy-violating content.

We have further conducted a statistical analysis of the correlation between the number of thinking tokens and both helpfulness and leakage scores. The correlations were weak in both cases, suggesting that longer chains of thought are not strongly associated with improved task performance or increased risk. This indicates that in this domain, lengthy reasoning traces may not be necessary — potentially offering cost advantages in agentic settings.

%%%%%%%%%%%%%%%%%%%%%%%%%%%%%%%%%%%%%%%%%%%%%%%%%%%%%
\paragraph{Computer Resources.} 
All tasks are trained and evaluated on a platform of 8 nodes with $8$ NVIDIA A100 GPUs on each node, and $80$ GB of memory for each GPU.
Each task requires between $8$ and $68$ hours to execute, depending on the model size.
