# Supplementary material for: Reinforcement Learning for Scalable and Trustworthy Intelligent Systems
Source: arXiv:2605.08378 source file (2026-05-08)
Supplement: Supplementary file 11 [file appendix_A.tex]

\section{Theoretical Results}

\subsection{Stationary Convergence of MaPPO}
\label{app:theo_converge}

Recall that 
\begin{equation}
\label{eq:mappo_loss_u}
\begin{aligned}
    \mathcal{L}_{\rm MaP}(\theta) ~=~& 
    \mathop{\mathbb{E}}_{( \mathbf{y}_{w}, \mathbf{y}_{l}, \mathbf{x})\sim\mathcal{D}} \Big[ -\log \sigma \Big( \beta\log \frac{\pi_{\theta}(\mathbf{y}_{w}|\mathbf{x})}{\pi_{\rm ref}(\mathbf{y}_{w}|\mathbf{x})} - \Delta_{r} \beta\log \frac{\pi_{\theta}(\mathbf{y}_{l}|\mathbf{x})}{\pi_{\rm ref}(\mathbf{y}_{l}|\mathbf{x})} \Big)\Big] \\
    ~=~& \mathop{\mathbb{E}}_{( \mathbf{y}_{w}, \mathbf{y}_{l}, \mathbf{x})\sim\mathcal{D}} \Big[ -\log \sigma (u) \Big].
\end{aligned}
\end{equation}

At the first-order stationary point (FOSP), the gradient of the loss with respect to $\theta$ becomes $0$. Thus, we have 
\begin{equation}
\label{eq:mappo_grad_0}
\begin{aligned}
    \nabla \mathcal{L}_{\rm MaP}(\theta) ~=~&
    \mathop{\mathbb{E}}_{( \mathbf{y}_{w}, \mathbf{y}_{l}, \mathbf{x})\sim\mathcal{D}} \Big[ -\beta (1-\sigma(u)) \Big( \nabla \log {\pi_{\theta}(\mathbf{y}_{w}|\mathbf{x})} - \Delta_{r} \nabla \log {\pi_{\theta}(\mathbf{y}_{l}|\mathbf{x})} \Big)\Big] = 0.
\end{aligned}
\end{equation}

Let the optimal policy be $\pi_{\star}$. The above equation holds when 
\begin{equation}
\label{eq:mappo_grad_inside_0}
\begin{aligned}
\nabla \log {\pi_{\star}(\mathbf{y}_{w}|\mathbf{x})} - \Delta_{r} \nabla \log {\pi_{\star}(\mathbf{y}_{l}|\mathbf{x})} ~=~ 0.
\end{aligned}
\end{equation}

Thus, the optimal policy achieves
\begin{equation}
\label{eq:mappo_opt}
\begin{aligned}
\log {\pi_{\star}(\mathbf{y}_{w}|\mathbf{x})} ~=~ \Delta_{r} \log {\pi_{\star}(\mathbf{y}_{l}|\mathbf{x})} + c,
\end{aligned}
\end{equation}
where $c$ is a scaling constant determined by the initialization. Thus, the model learns a stable log-linear relationship between preferred and less-preferred responses, scaled by the prior reward gap.

In DPO, the optimal policy at the FOSP is
\begin{equation}
\label{eq:dpo_opt}
\begin{aligned}
\log {\pi_{\star}(\mathbf{y}_{w}|\mathbf{x})} ~=~ \log {\pi_{\star}(\mathbf{y}_{l}|\mathbf{x})} + c.
\end{aligned}
\end{equation}
DPO converges to maximizing the log-odds between $\mathbf{y}_{w}$ and $\mathbf{y}_{l}$, but no inherent bound on the preference gap, which can lead to confidence degeneration. 
As training progresses, DPO may tend to decrease the likelihood of both $\mathbf{y}_{w}$ and $\mathbf{y}_{l}$ (the \emph{squeezing effect}), because there is no constraint on absolute probabilities -- only the relative gap matters.

MaPPO prevents overconfidence and instability by grounding optimization in the reward-based prior. 
The FOSP of MaPPO guarantees a bounded, calibrated log-probability ratio between $\mathbf{y}_{w}$ and $\mathbf{y}_{l}$. 
Naturally limits the \emph{squeezing effect} by scaling the impact of $\mathbf{y}_{l}$ via $\Delta_{r}$.
Therefore, MaPPO is theoretically more stable, especially for near-tie preference pairs and in large models where DPO can exacerbate miscalibration.

%%%%%%%%%%%%%%%%%%%%%%%%%%%%%%%%%%%%%%%%
\subsection{Lipschitz Stability}
\label{app:Lipschitz}

First, we list the standard assumptions for the analysis.
\begin{assumption}{\ }
\label{assum:bound}
\begin{enumerate}
% \item The norm of the score function is bounded as $\left\|\nabla \log \pi_\theta (\mathbf{y} | \mathbf{x}) \right\| \leq M$.
\item The score function is Lipschitz continuous as $\left\|\nabla \log \pi_\theta (\mathbf{y} | \mathbf{x}) - \nabla \log \pi_{\theta'} (\mathbf{y} | \mathbf{x}) \right\| \leq M_{g}$.
\end{enumerate}
\end{assumption}

Let the gradient operator be defined as
\begin{equation}
\label{eq:lip_mappo}
\begin{aligned}
\tau_{\theta} ~\coloneqq~  \nabla \mathcal{L}_{\rm MaP}(\theta).
\end{aligned}
\end{equation}

Then, the gradient operator $\tau$ is Lipschitz continuous with
\begin{equation}
\label{eq:lip_bound_mappo}
\begin{aligned}
\| \tau_{\theta} - \tau_{\theta'} \| \le L_{\rm MaP} \| \theta - \theta' \|,
\end{aligned}
\end{equation}
where $L_{\rm MaP} = \beta (1 - \sigma(u)) (1 + \Delta_{r}) M_{g} < \beta (1 + \Delta_{r}) M_{g}$.

\begin{proof}
We have
\begin{equation}
\begin{aligned}
\tau_{\theta} ~=~ -\beta (1-\sigma(u)) \Big( \nabla \log {\pi_{\theta}(\mathbf{y}_{w}|\mathbf{x})} - \Delta_{r} \nabla \log {\pi_{\theta}(\mathbf{y}_{l}|\mathbf{x})} \Big).
\end{aligned}
\end{equation}

The norm of the gradient difference is 
\begin{equation}
\begin{aligned}
\| \tau_{\theta} - \tau_{\theta'} \| ~=&~ \beta (1-\sigma(u)) \cdot \| \nabla \log {\pi_{\theta}(\mathbf{y}_{w}|\mathbf{x})} - \nabla \log {\pi_{\theta'}(\mathbf{y}_{w}|\mathbf{x})} \| \\
&+ \beta (1-\sigma(u)) \Delta_{r} \cdot \| \nabla \log {\pi_{\theta}(\mathbf{y}_{l}|\mathbf{x})} - \nabla \log {\pi_{\theta'}(\mathbf{y}_{l}|\mathbf{x})} \|.
\end{aligned}
\end{equation}

We have that $\sigma(u)$ is Lipschitz with constant $\frac{1}{4}$. Combining the $M_{g}$ Lipschitz of the score function $\nabla \log \pi_\theta (\mathbf{y} | \mathbf{x})$, we have
\begin{equation}
\begin{aligned}
\| \tau_{\theta} - \tau_{\theta'} \| \leq \beta (1 - \sigma(u)) (1 + \Delta_{r}) M_{g} \| \theta - \theta' \| ~\coloneqq~ L_{\rm MaP} \| \theta - \theta' \|.
\end{aligned}
\end{equation}
\end{proof}

In contrast, in DPO, the gradient is Lipschitz continuous as
\begin{equation}
\label{eq:lip_bound_dpo}
\begin{aligned}
\| \tau_{\theta} - \tau_{\theta'} \| \le L_{\rm DPO} \| \theta - \theta' \|,
\end{aligned}
\end{equation}
where $L_{\rm DPO} = 2\beta (1 - \sigma(u)) M_{g} < 2\beta M_{g}$. The Lipschitz constant of the gradients in DPO is larger than that in MaPPO, which shows the gradients have less stability in DPO.

With a formal upper bound on MaPPO's gradient variation, we show a clear theoretical justification for why MaPPO is less prone to instability and exploding confidence gaps, compared to DPO.
