# Supplementary material for: Reinforcement Learning for Scalable and Trustworthy Intelligent Systems
Source: arXiv:2605.08378 source file (2026-05-08)
Supplement: Supplementary file 12 [file appendix_B.tex]

\clearpage
\newpage
\section{Supplementary Experiments}
\label{app:Experiments}

\subsection{Supplementary Experimental Settings}
\label{mappo:sec:app_exp_setting}

\paragraph{Hyperparameter settings.} 
We follow the standard settings and list the hyperparameter details in the training process of MaPPO in Table \ref{table:hyper}. 
We keep the hyperparameter settings for different model series and model sizes, including Qwen2.5-\{1.5B, 3B, 7B\}-Instruct, Mistral-7B-Instruct, and Llama-3-8B-Instruct models. 

\begin{table}[!htbp]
\caption{Hyperparameter settings in MaPPO.}
\centering
 % \small
\label{table:hyper}
\begin{tabular}{l|lc}
\toprule[1.1pt]
% \hline
{Hyperparameter} & {Value} & {} \\
\midrule[1.1pt]
{global batch size} & {$128$} & { } \\
{learning rate $\eta$} & {$5\times 10^{-7}$} & { } \\
{warmup steps} & {$100$} & { } \\
{weight decay} & {$0.01$} & { } \\
{optimizer} & {AdamW} & { } \\
{KL weight $\beta$} & {$0.1$} & { } \\
{number of responses $n$} & {$8$} & { } \\
{temperature $T$} & {$1.0$} & { } \\
{precision} & {${\tt bfloat16}$} & { } \\
\bottomrule[1.1pt]
\end{tabular}
\end{table}

\begin{table}[!htbp]
\caption{Hyperparameter settings in DPO Variants.}
\centering
 % \small
\label{table:hyper_variants}
\begin{tabular}{l|lc}
\toprule[1.1pt]
{Hyperparameter} & {Value} & {} \\
\midrule[1.1pt]
{SimPO: $\gamma$} & {$1$} & { } \\
{IPO: $\beta$} & {$0.1$} & { } \\
{CPO: $\lambda$} & {$0.2$} & { } \\
\bottomrule[1.1pt]
\end{tabular}
\end{table}

In Table \ref{table:hyper_variants}, we list the extra hyperparameters in the reproduce of the DPO variants. 
The other hyperparameter settings keep the same in Table \ref{table:hyper}. 
Notably, we choose nearly the best hyperparameters for the other methods, and our reproduction achieves higher performances than the original or other reproduction reports on some benchmarks, \textit{e.g.}, SimPO on Arena-Hard. 

\paragraph{Computing Resources.} 
All tasks are trained and evaluated on a platform with $8$ NVIDIA A100 GPUs on each node, and $80$ GB of memory for each GPU. 
Each training task requires between $4$ and $20$ hours to execute, depending on the size of the model.

\subsection{Supplementary Results}
\label{mappo:app:supp_results}

\paragraph{Ablation Study on RMs.} 
As illustrated in Eq.~\ref{eq:prior_prob}, the prior is instantiated via a reward model (RM).
To better understand the role of RMs, we conduct an ablation study by integrating different open-source RMs into our framework, including BT model\footnote{https://huggingface.co/sfairXC/FsfairX-LLaMA3-RM-v0.1}, MoE model\footnote{https://huggingface.co/RLHFlow/ArmoRM-Llama3-8B-v0.1}, and uncertainty-aware model\footnote{https://huggingface.co/LxzGordon/URM-LLaMa-3.1-8B}. As shown in Table~\ref{table:RewardAblation_app}, the absolute performance of I-DPO varies considerably depending on the chosen RM. Importantly, across all settings, our proposed MaPPO plugin consistently boosts performance on AlpacaEval 2.0, Arena-Hard, and MT-Bench. These results highlight two key insights: (i) the choice of RM can influence the strength of supervision and the final outcomes, and (ii) MaPPO is robust to such variation, reliably enhancing DPO regardless of the underlying RM. This robustness underscores the generality and flexibility of our framework.

\begin{table}[!ht]
% \vspace{-4mm}
\caption{Ablation on reward models. $\uparrow$ indicates the higher the better.}
\centering
\label{table:RewardAblation_app}
\resizebox{\textwidth}{!}{%
\begin{tabular}{l|l|l|lll}
\toprule[1.1pt]
{Model} & {Reward Model} & {Method} & {AlpacaEval 2.0 $\uparrow$} & {Arena-Hard $\uparrow$} & {MT-Bench $\uparrow$} \\
\midrule[1.1pt]

\multirow{9}{*}{Qwen2.5-7B-IT}  
& \multirow{3}{*}{sfairXC/FsfairX-LLaMA3-RM-v0.1} 
& {IT} & {$27.03$}  & {$42.9$ }  & {$8.61$ } \\
& & {I-DPO} & {$33.80$} & {$46.9$} & {$\mathbf{8.55}$}\\
& & {+\textbf{MaPPO}} & {$\mathbf{39.10}$ $\textcolor{ForestGreen}{+5.30}$} & {$\mathbf{61.6}$ $\textcolor{ForestGreen}{+14.7}$} & {$8.54$ $\textcolor{Apricot}{-0.01}$}\\
\cline{2-6}
{}
& \multirow{3}{*}{RLHFlow/ArmoRM-Llama3-8B-v0.1} 
& {IT} & {$27.03$}  & {$42.9$ }  & {$8.61$ } \\
& & {I-DPO} & {$28.79$} & {$48.3$} & {$8.58$}\\
& & {+\textbf{MaPPO}} & {$\mathbf{31.56}$ $\textcolor{ForestGreen}{+2.77}$} & {$\mathbf{52.0}$ $\textcolor{ForestGreen}{+3.7}$} & {$\mathbf{8.60}$ $\textcolor{ForestGreen}{+0.02}$}\\

\cline{2-6}
{}  
& \multirow{3}{*}{LxzGordon/URM-LLaMa-3.1-8B} 
& {IT} & {$27.03$}  & {$42.9$ }  & {$8.61$ } \\
& & {I-DPO} & {$32.26$} & {$55.1$} & {$8.60$}\\
& & {+\textbf{MaPPO}} & {$\mathbf{36.17}$ $\textcolor{ForestGreen}{+3.91}$} & {$\mathbf{59.4}$ $\textcolor{ForestGreen}{+4.3}$} & {$\mathbf{8.62}$ $\textcolor{ForestGreen}{+0.02}$}\\

\midrule[1.1pt]

\multirow{9}{*}{Llama-3-8B-IT}  
& \multirow{3}{*}{sfairXC/FsfairX-LLaMA3-RM-v0.1} 
& {IT} & {$10.85$} &{$10.2$}&{$7.52$}\\
& & {I-DPO} & {${29.47}$} &{$25.6$ }&{$8.01$}\\
& & {+\textbf{MaPPO}} & {$\mathbf{32.68}$ $\textcolor{ForestGreen}{+3.21}$} & {$\mathbf{31.0}$ $\textcolor{ForestGreen}{+5.4}$} & {$\mathbf{8.04}$ $\textcolor{ForestGreen}{+0.03}$} \\
\cline{2-6}
{}  
& \multirow{3}{*}{RLHFlow/ArmoRM-Llama3-8B-v0.1} 
& {IT} & {$10.85$} &{$10.2$}&{$7.52$}\\
& & {I-DPO} & {$12.69$} &{$8.1$ }&{$7.44$}\\
& & {+\textbf{MaPPO}} & {$\mathbf{16.69}$ $\textcolor{ForestGreen}{+4.00}$} & {$\mathbf{16.4}$ $\textcolor{ForestGreen}{+8.3}$} & {$\mathbf{7.78}$ $\textcolor{ForestGreen}{+0.34}$} \\

\cline{2-6}
{}  
& \multirow{3}{*}{LxzGordon/URM-LLaMa-3.1-8B} 
& {IT} & {$10.85$} &{$10.2$}&{$7.52$}\\
& & {I-DPO} & {$25.61$} &{$30.4$ }&{$8.06$}\\
& & {+\textbf{MaPPO}} & {$\mathbf{27.83}$ $\textcolor{ForestGreen}{+2.22}$} & {$\mathbf{33.7}$ $\textcolor{ForestGreen}{+3.3}$} & {$\mathbf{8.10}$ $\textcolor{ForestGreen}{+0.04}$} \\

\bottomrule[1.1pt]
\end{tabular}
} % end resizebox
\end{table}

\begin{table}[!ht]
% \vspace{-4mm}
\caption{Comparison w/wo SFT-B and w/wo MaPPO. $\uparrow$ indicates the higher the better.}
\centering
  \small
\label{table:EvaluationICLR_app}
\begin{tabular}{l|l|lll}
\toprule[1.1pt]
% \hline
{Model} & {Method} & {AlpacaEval 2.0 $\uparrow$} & {Arena-Hard $\uparrow$} & {MT-Bench $\uparrow$} \\
\midrule[1.1pt]
\multirow{5}{*}{Qwen2.5-7B-IT} & {IT} & {$27.03$}  & {$42.9$ }  & {$8.61$ } \\
\cline{2-5}
{ } & {I-DPO} & {$33.80$} & {$46.9$} & {$\mathbf{8.55}$}\\
{ } & {+\textbf{MaPPO}} & {$\mathbf{39.10}$ $\textcolor{ForestGreen}{+5.30}$ ~$\textcolor{blue}{+5.30}$} & {$\mathbf{61.6}$ $\textcolor{ForestGreen}{+14.7}$ $\textcolor{blue}{+14.7}$} & {$8.54$ $\textcolor{Apricot}{-0.01}$ $\textcolor{blue}{-0.01}$} \\
\cline{2-5}
{ } & {+\textbf{SFT-B}} & {$51.36$\ \ $\textcolor{ForestGreen}{+17.56}$} & {$33.5$\ \ $\textcolor{Apricot}{-13.4}$} & {$8.01$ $\textcolor{Apricot}{-0.54}$} \\
{ } & {+\textbf{+MaPPO}} & {$\textbf{55.84}$ $\textcolor{ForestGreen}{+22.04}$ $\textcolor{blue}{+4.48}$} & {$\mathbf{43.5}$ ~$\textcolor{Apricot}{-3.4}$ ~$\textcolor{blue}{+10.0}$} & {$\mathbf{8.40}$ $\textcolor{Apricot}{-0.15}$ $\textcolor{blue}{+0.39}$}\\
\midrule[1.1pt]
\multirow{5}{*}{Llama-3-8B-IT} & {IT} & {$10.85$} &{$10.2$}&{$7.52$}\\
\cline{2-5}
{ } & {I-DPO} & {${29.47}$} &{$25.6$}&{$8.01$} \\
{ } & {+\textbf{MaPPO}} & {$\mathbf{32.68}$ $\textcolor{ForestGreen}{+3.21}$ $\textcolor{blue}{+3.21}$} & {$\mathbf{31.0}$ $\textcolor{ForestGreen}{+5.4}$ $\textcolor{blue}{+5.4}$} & {$\mathbf{8.04}$ $\textcolor{ForestGreen}{+0.03}$ $\textcolor{blue}{+0.03}$} \\
\cline{2-5}
{ } & {+\textbf{SFT-B}} & {$35.55$ ~$\textcolor{ForestGreen}{+6.08}$} & {$30.1$ ~$\textcolor{ForestGreen}{+4.5}$} & {$8.02$ ~$\textcolor{ForestGreen}{+0.01}$} \\
{ } & {+\textbf{+MaPPO}} & {$\mathbf{36.21}$ $\textcolor{ForestGreen}{+6.74}$ $\textcolor{blue}{+0.66}$} & {$\mathbf{31.5}$ $\textcolor{ForestGreen}{+5.9}$ $\textcolor{blue}{+1.4}$} & {$\mathbf{8.03}$ $\textcolor{ForestGreen}{+0.02}$ $\textcolor{blue}{+0.01}$} \\
\bottomrule[1.1pt]
\end{tabular}
\end{table}

\paragraph{Comparison with Other Methods.} 
We also compare our approach with complementary techniques, such as the method proposed by \cite{ren2024learning}, which introduces an additional SFT-based pre-processing (denoted as SFT-B) to mitigate the squeezing effect.
It is worthy to mention that our proposed method is compatible with SFT-B.

In Table~\ref{table:EvaluationICLR_app}, we use the \textcolor{blue}{blue} color to indicate the improvement with the MaPPO plugin, and the \textcolor{ForestGreen}{green} color to indicate the improvement compared to I-DPO. 
We find SFT-B alone can bring substantial gains in certain metrics but may also introduce trade-offs on others (e.g., lower Arena-Hard performance on Qwen2.5-7B). By contrast, when combined with MaPPO, the two methods operate jointly and achieve consistent improvements across most benchmarks. These findings demonstrate that MaPPO can be seamlessly integrated with diverse training strategies, further broadening its applicability in practice.
