# Supplementary material for: Reinforcement Learning for Scalable and Trustworthy Intelligent Systems
Source: arXiv:2605.08378 source file (2026-05-08)
Supplement: Supplementary file 13 [file appendix_discussion.tex]

\section{Further Discussions}
\label{app:Discussions}

%%%%%%%%%%%%%%%%%%%%%%%%%%%%%%%%%%%%%%%%
\subsection{Prior Function}
\label{app:Prior_Function}

In Bayes estimation, the prior distribution is usually constructed by experts with domain knowledge without an exception to avoid it \citep{jaynes2007prior}.
We choose a simple form in \eqref{eq:prior_prob}, which has the same structure as the widely used prior function \citep{blei2010probabilistic} and aligns with the softmax probability. 
This brings a very clean result in \eqref{eq:mappo_loss}.
In this paper, we offer an effective function with good performances and concise formulation.
We bring the MaP design into the DPO pipeline, and the prior function construction is not the aim of this paper.
Other function choices that are designed by domain experts are also acceptable and open to be used.

On the other hand, we perform ablation studies on reward models in Appendix \ref{mappo:app:supp_results}, which shows the robustness to different reward signals.

%%%%%%%%%%%%%%%%%%%%%%%%%%%%%%%%%%%%%%%%
\subsection{Recent RL Methods}
\label{app:rl_methods}

In addition to the methods discussed in the introduction section, several recent variants of RL methods for LLMs further contextualize the landscape in which PO operates. 
DAPO \citep{yu2025dapo} introduces a scalable RL system that integrates data selection, clip-higher, overlong reward shaping, and token-level loss into a unified framework, demonstrating strong empirical performance at scale. 
GSPO \citep{zheng2025group} generalizes sequence-level policy optimization to groupwise preference structures, enabling the use of ranked or collectively generated signals and thereby broadening the applicability of RL methods into mixture-of-experts (MoE) architectures. 
PRO \citep{guo2025proximalized} proposes a proximalized formulation of preference optimization that decomposes preference signals into stable update components, allowing the method to accommodate diverse feedback modalities while improving optimization stability. 
Together, these approaches represent the most recent advances in preference optimization and RL post-training, situating MaPPO alongside them highlights its complementary role as a principled, prior-informed extension that remains compatible with the post-training pipelines. 
An interesting direction for future work is exploring how prior knowledge can be integrated into these RL methods.
