# Supplementary material for: Reinforcement Learning for Scalable and Trustworthy Intelligent Systems
Source: arXiv:2605.08378 source file (2026-05-08)
Supplement: Supplementary file 14 [file appendix_example.tex]

\clearpage
\newpage
\section{Supplementary Examples}
\label{app:Supplementary_Examples}

\begin{figure}[!htbp]
\begin{tcolorbox}[title=Prompt~$\mathbf{x}$,fonttitle=\bfseries, boxrule=0.5mm]
Solve the following math problem step-by-step. Simplify your answer as much as possible. Present your final answer as \boxed{Your Answer}. If the sum of two positive integers is 22 and the difference of their squares is 44, what is the product of the two integers?
\end{tcolorbox}
\end{figure}

%%%%%%%%%%%%%%%%%%%%%%%%%%%%%%%%%%%%%%%%
\newpage
\subsection{Before Preference Optimization}
\begin{figure}[!htbp]
\begin{tcolorbox}[colback=green!5, colframe=black!60!green!45, title={\textbf{Response}~$\mathbf{y}_{w}$, $r=0.93$}, fonttitle=\bfseries, boxrule=0.5mm]
To solve this problem step-by-step, let's denote the two positive integers as \(x\) and \(y\) with \(x > y\).

Step 1: Set Up Equations

~~~~Given:

~~~~~~~~1. The sum of the two integers: \(x + y = 22\)

~~~~~~~~2. The difference of their squares: \(x^2 - y^2 = 44\)

Step 2: Factorize the Difference of Squares
Recall that the difference of squares can be factored as:
\[ x^2 - y^2 = (x + y)(x - y) \]
Substitute the given sum \(x + y = 22\) into the factored form:
\[ 44 = 22(x - y) \]

Step 3: Solve for \(x - y\)
Divide both sides by 22:
\[ x - y = 2 \]

Step 4: Solve the System of Linear Equations
Now, we have the system:
1. \(x + y = 22\)
2. \(x - y = 2\)

Add these two equations to eliminate \(y\):
\[ (x + y) + (x - y) = 22 + 2 \]
\[ 2x = 24 \]
\[ x = 12 \]

Substitute \(x = 12\) back into the first equation to find \(y\):
\[ 12 + y = 22 \]
\[ y = 10 \]

Step 5: Calculate the Product
The product of the two integers \(x\) and \(y\) is:
\[ x \cdot y = 12 \cdot 10 = 120 \]

Final Answer
\[ \boxed{120} \] 
\end{tcolorbox}
\end{figure}

\begin{figure}[!htbp]
\begin{tcolorbox}[colback=red!5, colframe=black!60!red!45, title={\textbf{Response}~$\mathbf{y}_{l}$, $r=0.90$}, fonttitle=\bfseries, boxrule=0.5mm]
To solve this problem step-by-step, let's denote the two positive integers as \(x\) and \(y\), where \(x > y\). We are given two conditions:

1. The sum of the two integers is 22:
   \[ x + y = 22 \]

2. The difference of their squares is 44:
   \[ x^2 - y^2 = 44 \]

We can use the identity for the difference of squares, \(x^2 - y^2 = (x + y)(x - y)\), to rewrite the second equation. Substituting \(x + y = 22\) into the identity gives:
\[
(x + y)(x - y) = 44 \implies 22(x - y) = 44
\]
Dividing both sides by 22:
\[
x - y = 2
\]

Now we have a system of linear equations:
\[
\begin{cases}
x + y = 22 \\
x - y = 2
\end{cases}
\]

Adding these two equations eliminates \(y\):
\[
(x + y) + (x - y) = 22 + 2 \implies 2x = 24 \implies x = 12
\]

Substituting \(x = 12\) back into the first equation to solve for \(y\):
\[
12 + y = 22 \implies y = 10
\]

Thus, the two integers are \(x = 12\) and \(y = 10\).

To find the product of the two integers:
\[ xy = 12 \times 10 = 120 \]

Therefore, the product of the two integers is \boxed{120}. 
\end{tcolorbox}
\begin{center}
\caption{Before MLE optimization, the model consistently generates high-quality (high rewards) answers $\mathbf{y}_{w}$ and $\mathbf{y}_{l}$ with prompt $\mathbf{x}$.}
\end{center}
\end{figure}

%%%%%%%%%%%%%%%%%%%%%%%%%%%%%%%%%%%%%%%%%%%
\clearpage
\newpage
\subsection{After MLE Optimization}

\begin{figure}[!htbp]
\begin{tcolorbox}[breakable,colback=green!5, colframe=black!60!green!45, title={\textbf{Response}~$\mathbf{y}_{w}$, $r=0.87$}, fonttitle=\bfseries, boxrule=0.5mm]
To solve the given problem, we'll proceed through the following steps systematically:

Given:

~~~~1. The sum of two positive integers \( x \) and \( y \) is 22.

~~~~2. The difference of their squares is 44.

We need to determine the product of these two integers.

Step-by-Step Solution:

1. Setting up Equations:
   
   - From the first condition: 
     \[
     x + y = 22
     \]
   - From the second condition (expressing the difference of squares):
     \[
     x^2 - y^2 = 44
     \]
   
   We know that \( x^2 - y^2 \) can be factored using the difference of squares formula:
     \[
     x^2 - y^2 = (x+y)(x-y)
     \]

2. Substitute \( x + y \):
   
   - Using the known value from equation (1) in the factored form of the difference of squares:
     \[
     x^2 - y^2 = (x+y)(x-y) \implies 44 = 22(x-y)
     \]
   - Solve for \( x - y \):
     \[
     22(x - y) = 44 \implies x - y = 2
     \]

3. Solving the System of Linear Equations:
   
   - Now, we have the system of equations:
     \[
     x + y = 22
     \]
     \[
     x - y = 2
     \]
   - Add these two equations to eliminate \( y \):
     \[
     (x + y) + (x - y) = 22 + 2
     \]
     \[
     2x = 24 \implies x = 12
     \]
   - Substitute \( x = 12 \) back into \( x + y = 22 \) to find \( y \):
     \[
     12 + y = 22 \implies y = 10
     \]
\end{tcolorbox}
\end{figure}

\clearpage
\newpage
\begin{figure}[!htbp]
\begin{tcolorbox}[breakable,colback=green!5, colframe=black!60!green!45, title={\textbf{Response}~$\mathbf{y}_{w}$, $r=0.87$}, fonttitle=\bfseries, boxrule=0.5mm]
4. Finding the Product:
   
   - With \( x = 12 \) and \( y = 10 \), calculate the product:
     \[
     xy = 12 \times 10 = 120
     \]

Thus, the product of the two integers is \boxed{120}.
\end{tcolorbox}
\end{figure}

\begin{figure}[!htbp]
\begin{tcolorbox}[colback=red!5, colframe=black!60!red!45, title={\textbf{Response}~$\mathbf{y}_{l}$, $r=0.43$}, fonttitle=\bfseries, boxrule=0.5mm]
Step 1: Interpret the problem and set up equations based on the given information.
Given that the sum of two positive integers is 22 and the difference of their squares is 44, we need to find these integers and subsequently their product.

Let's denote the two integers as \(a\) and \(b\) such that \(a > b\), to simplify handling the difference and sum relationships given directly without specifying which integer represents \(a\) or \(b\) in terms of being greater than the other directly addresses addressing conditions related directly to interpreting the context regarding how the operations (sum, difference of squares) relate between two specified integers, based on the given descriptions for solving in the context presented, focusing on correctly interpreting and directly addressing the specific requirements as outlined for accurately proceeding with solving based on the given details, to correctly proceed according to provided instructions and the nature of solving based on the specifications given for dealing with the described conditions around the operation outcomes involving the integers in question.
\[ \]
Step 2: Translate the given conditions into mathematical equations.

~~~~- The sum of the two integers equals 22: \(a + b = 22\).

~~~~- The difference of their squares equals 44: \(a^2 - b^2 = 44\).
\[ \]
Step 3: Utilize algebraic identities for simplification.
From the second equation, apply the algebraic identity for the difference of squares: 
\[a^2 - b^2 = (a + b)(a - b)\]
Thus, substituting in the known value for \(a + b\):
\[(a + b)(a - b) = 44 \implies 22(a - b) = 44.\]

Step 4: Solve for \(a - b\).
Divide both sides by 22:
\[a - b = 2.\]

Step 5: Solve the system of linear equations.
We now have two simultaneous equations:

~~~~1. \(a + b = 22\)

~~~~2. \(a - b = 2\)

Add the two equations together to eliminate \(b\):
\[(a + b) + (a - b) = 22 + 2 \implies 2a = 24 \implies a = 12.\]
\end{tcolorbox}
\end{figure}

\clearpage
\newpage
\begin{figure}[!htbp]
\begin{tcolorbox}[colback=red!5, colframe=black!60!red!45, title={\textbf{Response}~$\mathbf{y}_{l}$, $r=0.43$}, fonttitle=\bfseries, boxrule=0.5mm]
Substitute \(a = 12\) back into the first equation to solve for \(b\):
\[12 + b = 22 \implies b = 10.\]

Step 6: Find the product of \(a\) and \(b\).
The product of the two integers \(a\) and \(b\) is:
\[ab = 12 \times 10 = 120.\]

Step 7: Box the final answer.
\[\boxed{120}\]

\end{tcolorbox}
\begin{center}
\caption{After MLE optimization, the model degenerates, and the outputs $\mathbf{y}_{w}$ and $\mathbf{y}_{l}$ become verbose (low rewards) with prompt $\mathbf{x}$.}
\end{center}
\end{figure}

\clearpage
\newpage
\subsection{After MaP Optimization}

\begin{figure}[!htbp]
\begin{tcolorbox}[colback=green!5, colframe=black!60!green!45, title={\textbf{Response}~$\mathbf{y}_{w}$, $r=0.94$}, fonttitle=\bfseries, boxrule=0.5mm]
To solve this problem step-by-step, let's denote the two positive integers by \(x\) and \(y\), where without loss of generality, we assume \(x > y\).

Given:

~~~~1. The sum of the two integers: \(x + y = 22\)

~~~~2. The difference of their squares: \(x^2 - y^2 = 44\)
\[\]
Step 1: Express the Difference of Squares

~~~~We know from algebra that:
\[ x^2 - y^2 = (x + y)(x - y) \]

~~~~Given \(x + y = 22\), we substitute this into the equation:
\[ 44 = 22(x - y) \]

Step 2: Solve for \(x - y\)

~~~~Divide both sides by 22:
\[ x - y = 2 \]

Step 3: Solve the System of Linear Equations

~~~~Now, we have a system of linear equations:

~~~~~~~~1. \(x + y = 22\)

~~~~~~~~2. \(x - y = 2\)

~~~~Add these two equations to eliminate \(y\):
\[ (x + y) + (x - y) = 22 + 2 \]
\[ 2x = 24 \]
\[ x = 12 \]

~~~~Subtract the second equation from the first to eliminate \(x\):
\[ (x + y) - (x - y) = 22 - 2 \]
\[ 2y = 20 \]
\[ y = 10 \]
\end{tcolorbox}
\end{figure}

\clearpage
\newpage
\begin{figure}[!htbp]
\begin{tcolorbox}[colback=green!5, colframe=black!60!green!45, title={\textbf{Response}~$\mathbf{y}_{w}$, $r=0.94$}, fonttitle=\bfseries, boxrule=0.5mm]
Step 4: Calculate the Product of the Two Integers

~~~~Now that we have \(x = 12\) and \(y = 10\), we find their product:
\[ xy = 12 \times 10 = 120 \]

~~~~Thus, the product of the two integers is:
\[\boxed{120}\]
\end{tcolorbox}
\end{figure}

\begin{figure}[!htbp]
\begin{tcolorbox}[colback=red!5, colframe=black!60!red!45, title={\textbf{Response}~$\mathbf{y}_{l}$, $r=0.88$}, fonttitle=\bfseries, boxrule=0.5mm]
To solve this problem, we'll use algebraic methods to represent the given conditions and then solve for the integers. Here are the steps:

1. Define Variables:
   
~~~~Let the two positive integers be \(x\) and \(y\), with \(x > y\).
\[\]
2. Set Up Equations Based on Given Information:
   
~~~~- The sum of the two integers is 22:
     \[
     x + y = 22
     \]
   
~~~~- The difference of their squares is 44:
     \[
     x^2 - y^2 = 44
     \]

3. Factor the Difference of Squares:
   
~~~~Recall that \(x^2 - y^2\) can be factored as \((x + y)(x - y)\). Therefore:
   \[
   (x + y)(x - y) = 44
   \]
~~~~Substitute \(x + y = 22\) into the equation:
   \[
   22(x - y) = 44
   \]

4. Solve for \(x - y\):
   
~~~~Divide both sides by 22:
   \[
   x - y = 2
   \]
\end{tcolorbox}
\end{figure}

\clearpage
\newpage
\begin{figure}[!htbp]
\begin{tcolorbox}[colback=red!5, colframe=black!60!red!45, title={\textbf{Response}~$\mathbf{y}_{l}$, $r=0.88$}, fonttitle=\bfseries, boxrule=0.5mm]
5. Set Up a System of Linear Equations:

~~~~We now have the system:
   \[
   \begin{cases}
   x + y = 22 \\
   x - y = 2
   \end{cases}
   \]

6. Add the Two Equations to Solve for \(x\):

~~~~Adding the equations eliminates \(y\):
   \[
   (x + y) + (x - y) = 22 + 2
   \]
~~~~Simplifies to:
   \[
   2x = 24 \implies x = 12
   \]

7. Substitute \(x = 12\) Back to Find \(y\):
   
~~~~Using \(x + y = 22\):
   \[
   12 + y = 22 \implies y = 10
   \]

8. Calculate the Product of the Two Integers:

~~~~The product of \(x\) and \(y\) is:
   \[
   x \cdot y = 12 \cdot 10 = 120
   \]
The answer is
 \[\boxed{120}\]

\end{tcolorbox}
\begin{center}
\caption{After MaP optimization, the model consistently generates high quality outputs with prompt $\mathbf{x}$.}
\end{center}
\end{figure}
