# Supplementary material for: Reinforcement Learning for Scalable and Trustworthy Intelligent Systems
Source: arXiv:2605.08378 source file (2026-05-08)
Supplement: Supplementary file 15 [file rebuttal.tex]

\section*{Rebuttal}

\subsection*{Reviewer 2SVh}

We sincerely appreciate the reviewer’s valuable and constructive feedback. In accordance with the suggestion, we have added a paragraph in Appendix D.2 that discusses and categorizes several recent RL-based methods for LLM post-training, including DAPO [1], GSPO [2], and PRO [3]. We thank the reviewer for the positive comments and for helping us improve the clarity and completeness of the manuscript.


%%%%%%%%%%%%%%%%%%%%%%%%%%%%%%%%%%%%%%%%%%%%%%%%%%%%%%%%%%%%
\subsection*{Reviewer U27W}

Copy wQhG's Q1. %Do we need to do ablation studies on different reward models (quality of the prior reward)?

%%%%%%%%%%%%%%%%%%%%%%%%%%%%%%%%%%%%%%%%%%%%%%%%%%%%%%%%%%%%
\subsection*{Reviewer wQhG}

Q1. 

We thank the reviewer for bringing this concern to our attention. We would like to emphasize that our prior design does not rely on introducing additional heuristics. Instead, we simply leverage a widely used open-source reward model (sfairXC/FsfairX-LLaMA3-RM-v0.1) to provide supervision, and this already leads to strong empirical results. Moreover, our framework is flexible with different reward signals: different reward models can be seamlessly integrated. To demonstrate this, we evaluate two alternative models (MoE model RLHFlow/ArmoRM-Llama3-8B-v0.1, and uncertainty-aware model LxzGordon/URM-LLaMa-3.1-8B) with further comparisons.

Table~\ref{table:RewardAblation} shows that although I-DPO performance can vary depending on the reward model, our method robustly and consistently improves the results across all reward models (different prior reward signals).

\begin{table}[!ht]
% \vspace{-4mm}
\caption{Main evaluation results on three standard benchmarks. $\uparrow$ indicates the higher the better.}
\centering
\label{table:RewardAblation}
\resizebox{\textwidth}{!}{%
\begin{tabular}{l|l|l|lll}
\toprule[1.1pt]
{Model} & {Reward Model} & {Method} & {AlpacaEval 2.0 $\uparrow$} & {Arena-Hard $\uparrow$} & {MT-Bench $\uparrow$} \\
\midrule[1.1pt]

\multirow{9}{*}{Qwen2.5-7B-IT}  
& \multirow{3}{*}{sfairXC/FsfairX-LLaMA3-RM-v0.1} 
& {IT} & {$27.03$}  & {$42.9$ }  & {$8.61$ } \\
& & {I-DPO} & {$33.80$} & {$46.9$} & {$\mathbf{8.55}$}\\
& & {+\textbf{MaPPO}} & {$\mathbf{39.10}$ $\textcolor{ForestGreen}{+5.30}$} & {$\mathbf{61.6}$ $\textcolor{ForestGreen}{+14.7}$} & {$8.54$ $\textcolor{Apricot}{-0.01}$}\\
\cline{2-6}
{}
& \multirow{3}{*}{RLHFlow/ArmoRM-Llama3-8B-v0.1} 
& {IT} & {$27.03$}  & {$42.9$ }  & {$8.61$ } \\
& & {I-DPO} & {$28.79$} & {$48.3$} & {$8.58$}\\
& & {+\textbf{MaPPO}} & {$\mathbf{31.56}$ $\textcolor{ForestGreen}{+2.77}$} & {$\mathbf{52.0}$ $\textcolor{ForestGreen}{+3.7}$} & {$\mathbf{8.60}$ $\textcolor{ForestGreen}{+0.02}$}\\

\cline{2-6}
{}  
& \multirow{3}{*}{LxzGordon/URM-LLaMa-3.1-8B} 
& {IT} & {$27.03$}  & {$42.9$ }  & {$8.61$ } \\
& & {I-DPO} & {$32.26$} & {$55.1$} & {$8.60$}\\
& & {+\textbf{MaPPO}} & {$\mathbf{36.17}$ $\textcolor{ForestGreen}{+3.91}$} & {$\mathbf{59.4}$ $\textcolor{ForestGreen}{+4.3}$} & {$\mathbf{8.62}$ $\textcolor{ForestGreen}{+0.02}$}\\

\midrule[1.1pt]

\multirow{9}{*}{Llama-3-8B-IT}  
& \multirow{3}{*}{sfairXC/FsfairX-LLaMA3-RM-v0.1} 
& {IT} & {$10.85$} &{$10.2$}&{$7.52$}\\
& & {I-DPO} & {${29.47}$} &{$25.6$ }&{$8.01$}\\
& & {+\textbf{MaPPO}} & {$\mathbf{32.68}$ $\textcolor{ForestGreen}{+3.21}$} & {$\mathbf{31.0}$ $\textcolor{ForestGreen}{+5.4}$} & {$\mathbf{8.04}$ $\textcolor{ForestGreen}{+0.03}$} \\
\cline{2-6}
{}  
& \multirow{3}{*}{RLHFlow/ArmoRM-Llama3-8B-v0.1} 
& {IT} & {$10.85$} &{$10.2$}&{$7.52$}\\
& & {I-DPO} & {$12.69$} &{$8.1$ }&{$7.44$}\\
& & {+\textbf{MaPPO}} & {$\mathbf{16.69}$ $\textcolor{ForestGreen}{+4.00}$} & {$\mathbf{16.4}$ $\textcolor{ForestGreen}{+8.3}$} & {$\mathbf{7.78}$ $\textcolor{ForestGreen}{+0.34}$} \\

\cline{2-6}
{}  
& \multirow{3}{*}{LxzGordon/URM-LLaMa-3.1-8B} 
& {IT} & {$10.85$} &{$10.2$}&{$7.52$}\\
& & {I-DPO} & {$25.61$} &{$30.4$ }&{$8.06$}\\
& & {+\textbf{MaPPO}} & {$\mathbf{27.83}$ $\textcolor{ForestGreen}{+2.22}$} & {$\mathbf{33.7}$ $\textcolor{ForestGreen}{+3.3}$} & {$\mathbf{8.10}$ $\textcolor{ForestGreen}{+0.04}$} \\

\bottomrule[1.1pt]
\end{tabular}
} % end resizebox
\end{table}
% \begin{table}[!ht]
% \vspace{-4mm}
% \caption{Main evaluation results on three standard benchmarks. $\uparrow$ indicates the higher the better.}
% \centering
% \label{table:RewardAblation}
% \begin{tabular}{l|l|lll}
% \toprule[1.1pt]
% % \hline
% {Model} &{Method} & {AlpacaEval 2.0 $\uparrow$} & {Arena-Hard $\uparrow$} & {MT-Bench $\uparrow$} \\
% \midrule[1.1pt]
% \multirow{5}{*}{Qwen2.5-7B-Instruct}  &{IT} & {$27.03$}  & {$42.9$ }  & {$8.61$ } \\
% \cline{2-5}
% { } & {I-DPO} & {$33.80$} & {$46.9$} & {$\mathbf{8.55}$}\\
% { } & {+\textbf{MaPPO}} & {$\mathbf{39.10}$ $\textcolor{ForestGreen}{+5.30}$} & {$\mathbf{61.6}$ $\textcolor{ForestGreen}{+14.7}$} & {$8.54$ $\textcolor{Apricot}{-0.01}$}\\

% \midrule[1.1pt]
% \multirow{5}{*}{Llama-3-8B-Instruct} & {IT} & {$10.85$} &{$10.2$}&{$7.52$}\\
% \cline{2-5}
% { } & {I-DPO} & {${29.47}$} &{$25.6$ }&{$8.01$}\\
% { } & {+\textbf{MaPPO}} & {$\mathbf{32.68}$ $\textcolor{ForestGreen}{+3.21}$} & {$\mathbf{31.0}$ $\textcolor{ForestGreen}{+5.4}$} & {$\mathbf{8.04}$ $\textcolor{ForestGreen}{+0.03}$} \\

% \bottomrule[1.1pt]
% \end{tabular}
% \end{table}

Q2.

We thank the reviewer for this valuable suggestion. Following the approach outlined in [1], we treat it as a compatible module and seamlessly incorporate MaPPO, illustrating that the two approaches can operate jointly without conflict. 
In Table~\ref{table:EvaluationICLR}, we use the \textcolor{blue}{blue} color to indicate the improvement with the MaPPO plugin, and the \textcolor{ForestGreen}{green} color to indicate the improvement compared to I-DPO. 
The results show that MaPPO generally enhances training stability for both I-DPO and with the presence of SFT pre-processing in [1].
%改了一下我不知道下面的还是不是draft。。。
%We follow the methods mentioned in [1]. Additional, we plugin MaPPO into the methods, which result in Table \ref{table:EvaluationICLR}. We could figure out that generally MaPPO could help to stabilize the training even with the presence of SFT pre-processing.
%写得更详细,改写得学术一点，这只是个draft!!!

\begin{table}[!ht]
% \vspace{-4mm}
\caption{Main evaluation results on three standard benchmarks. $\uparrow$ indicates the higher the better.}
\centering
 % \small
\label{table:EvaluationICLR}
\begin{tabular}{l|l|lll}
\toprule[1.1pt]
% \hline
{Model} & {Method} & {AlpacaEval 2.0 $\uparrow$} & {Arena-Hard $\uparrow$} & {MT-Bench $\uparrow$} \\
\midrule[1.1pt]
\multirow{5}{*}{Qwen2.5-7B-IT} & {IT} & {$27.03$}  & {$42.9$ }  & {$8.61$ } \\
\cline{2-5}
{ } & {I-DPO} & {$33.80$} & {$46.9$} & {$\mathbf{8.55}$}\\
{ } & {+\textbf{MaPPO}} & {$\mathbf{39.10}$ $\textcolor{ForestGreen}{+5.30}$ ~$\textcolor{blue}{+5.30}$} & {$\mathbf{61.6}$ $\textcolor{ForestGreen}{+14.7}$ $\textcolor{blue}{+14.7}$} & {$8.54$ $\textcolor{Apricot}{-0.01}$ $\textcolor{blue}{-0.01}$} \\
\cline{2-5}
{ } & {+\textbf{SFT-B}} & {$51.36$\ \ $\textcolor{ForestGreen}{+17.56}$} & {$33.5$\ \ $\textcolor{Apricot}{-13.4}$} & {$8.01$ $\textcolor{Apricot}{-0.54}$} \\
{ } & {+\textbf{SFT-B +MaPPO}} & {$\textbf{55.84}$ $\textcolor{ForestGreen}{+22.04}$ $\textcolor{blue}{+4.48}$} & {$\mathbf{43.5}$ ~$\textcolor{Apricot}{-3.4}$ ~$\textcolor{blue}{+10.0}$} & {$\mathbf{8.40}$ $\textcolor{Apricot}{-0.15}$ $\textcolor{blue}{+0.39}$}\\
\midrule[1.1pt]
\multirow{5}{*}{Llama-3-8B-IT} & {IT} & {$10.85$} &{$10.2$}&{$7.52$}\\
\cline{2-5}
{ } & {I-DPO} & {${29.47}$} &{$25.6$}&{$8.01$} \\
{ } & {+\textbf{MaPPO}} & {$\mathbf{32.68}$ $\textcolor{ForestGreen}{+3.21}$ $\textcolor{blue}{+3.21}$} & {$\mathbf{31.0}$ $\textcolor{ForestGreen}{+5.4}$ $\textcolor{blue}{+5.4}$} & {$\mathbf{8.04}$ $\textcolor{ForestGreen}{+0.03}$ $\textcolor{blue}{+0.03}$} \\
\cline{2-5}
{ } & {+\textbf{SFT-B}} & {$35.55$ $\textcolor{ForestGreen}{+6.08}$} & {$30.1$ $\textcolor{ForestGreen}{+4.5}$} & {$8.02$ $\textcolor{ForestGreen}{+0.01}$} \\
{ } & {+\textbf{SFT-B +MaPPO}} & {$\mathbf{36.21}$ $\textcolor{ForestGreen}{+6.74}$ $\textcolor{blue}{+0.66}$} & {$\mathbf{31.5}$ $\textcolor{ForestGreen}{+5.9}$ $\textcolor{blue}{+1.4}$} & {$\mathbf{8.03}$ $\textcolor{ForestGreen}{+0.02}$ $\textcolor{blue}{+0.01}$} \\
\bottomrule[1.1pt]
\end{tabular}
\end{table}


Q3. 

We thank the reviewer for bringing this valuable observation. We clarify that this might be a misunderstanding. 
In Eq. 9, the logarithm is always applied to the probability ratio $\frac{\pi_\theta(y_w \mid x)}{\pi_\text{ref}(y_w \mid x)}$, which are strictly positive and lie in the interval $(0,1)$. Therefore, there is no risk of encountering negative inputs for the logarithm.
Compared to SFT, the entire $\log \sigma(\cdot)$ is added instead of $\sigma(\cdot)$.
Considering the monotonicity of \emph{outer} $\log \sigma(\cdot)$ over $(-\inf, 0)$, we further introduce Eq. 10 to explicitly connect SFT and MaP, where SFT emerges as a special case of our framework.
We make a general example to explain it explicitly. Let $f(\cdot)$ is strictly increasing function. The optimization problem ${\rm max}~L(\theta)$ has the same solution with respect to $\theta$ as ${\rm max}~f(L(\theta))$.

% (We will revise the text to make this point clearer and avoid possible confusion.) %场面话233

[1] Ren, Yi, and Danica J. Sutherland. Learning Dynamics of LLM Finetuning. ICLR 2025.
